# Supplementary material for: Multidisciplinary learning through collective performance favors decentralization
Source: arXiv:2208.11618 ancillary file (2023-08-14)
Supplement: Supplementary file 1 [file SI_Appendix.pdf]

# Supplementary Information for

## Indirect social learning through collective performance favors decentralization

John Meluso and Laurent Hébert-Dufresne

Corresponding Author: John Meluso

E-mail: [john.meluso@uvm.edu](mailto:john.meluso@uvm.edu)

### This PDF file includes:

Supplementary text

Figs. S1 to S11

Tables S1 to S4

Legends for Dataset S1 to S5

SI References

### Other supplementary materials for this manuscript include the following:

Datasets S1 to S5

## Supporting Information Text

### 1. Task measures

We constructed four measures to control for different qualities that describe tasks. These qualities are grounded in the different types of tasks identified by McGrath (1), which underlie studies of collective intelligence (2, 3) and are recommended for the study of transactive memory systems (4, 5). The four qualities are exploration difficulty, exploitation difficulty, neighborhood interdependence, and neighborhood alignment. An exploration difficulty (1—the integral of the task) measures the probability of finding better-performing solutions over the entire decision space. An exploitation difficulty (the number of peaks in the task) measures the likelihood that the team will randomly land on a peak in the task landscape with the best value. An interdependence difficulty (the average correlation between agents’ neighborhood performances) measures how likely a change in one agent’s neighborhood is to affect the neighborhood performance of another agent. Last, an alignment difficulty (the average difference between agents’ neighborhood performances) measures how likely agents’ changes are to produce commensurate changes for other agents. The follow sections motivate and define these measures.

**a. Exploration difficulty: 1 - integral of the task.** Exploration difficulty resembles the difficulty of generating new ideas or plans creatively (1). In our formulation, when agents can explore the entire decision space (search radius  $r = 1.0$ ), the relative position of each  $x_i$  does not matter. Random selection of each  $x_i$  effectively yields a probability distribution for different performance values. As a result, tasks that are more difficult for exploration are those for which there is a lower probability of finding a good performance value. In this work, performance values are “better” the closer they are to 1. So, we can measure the exploration difficulty of each task by calculating its expected value (through integration) over every  $x_i \in X$  on the domain  $[0, 1]$  and subtracting it from 1 as follows:

$$q_1(h(\vec{x})) = 1 - \int_X h(\vec{x}) d\vec{x}. \quad [1]$$

We calculated the integral for each task through Monte Carlo integration, that is, by generating 100 random vectors  $\vec{x}$ , calculating  $h(\vec{x})$  for each, and averaging their results. Subtracting the resulting value from one gave us the exploration difficulty.

**b. Exploitation difficulty: number of peaks in task.** This quality derives from choose tasks (1). Tasks with more peaks are often described as making it more difficult or complex to select the best answer (6–8), particularly when individuals are limited to moving to adjacent locations (as with a search radius  $r = 0.01$ ). So the second difficulty measure we define is the number of peaks in each task. The tasks we defined above are simple enough that we can analytically determine the number of peaks in each task by their shapes and frequencies. Many tasks only have one peak, or have a continuous ridge of best values (as with the maximum function, task aa) for which we set the number of peaks to 1 as well. On the other hand, those with sinusoidal forms can have many peaks in each dimension, which can yield  $10^{30}$  of more peaks for networks with large numbers of connections and degree frequencies. So our second measure of difficulty is:

$$q_2(h(\vec{x})) = \text{number of peaks}. \quad [2]$$

**c. Interdependence between task neighborhoods.** Execution tasks involve “coordination between members” (1, p.65). Tasks in which individuals actions are more interdependent require greater coordination, while those in which individuals actions are less interdependent require less coordination. Thus, we also measure how interdependent agents are by calculating the Spearman correlation coefficient  $r_s$  (9) between every pair of agents and averaging those coefficients. This captures how much agents affect each other when they make a change, and therefore measures how much control each agent has over their own outcomes given the influences of the others they indirectly interact with. This gives:

$$q_3(h(\vec{x})) = \frac{1}{n^2} \sum_{i,j} r_s(g_i, g_j) \quad [3]$$

Again, we generated 100 random vectors  $\vec{x}$  and entered these vectors into the neighborhood functions  $g_i$  and  $g_j$  to generate  $r_s$  for each pair of nodes.

**d. Alignment Between Task Neighborhoods.** Last, agents actions need not be aligned with one another. Many tasks involve negotiation to resolve conflicts or advance mixed motives (1). In our formulations, a great change for one agent might produce only small gains for their neighbor. Or in a few cases, an improvement for one agent could result in degraded performance for their neighbor, potentially leading to adaptive dynamics where agents compete (only the non-commutative tasks—that is, the high- and low-degree swinging tasks s, u, w, & y—see this among the tasks we constructed above). While the intent of this work was not primarily to explore these dynamics, we controlled for misalignment between agent interests by measuring how different their neighborhood performances are from one another on average:

$$q_4(h(\vec{x})) = \frac{1}{n^2} \sum_{i,j} \left( 1 - \frac{1}{v} \sum_v |g_i - g_j| \right) \quad [4]$$

where agents that are completely aligned have paired values of 1, and completely misaligned have values of 0. Here, too, we generated  $v = 100$  random vectors  $\vec{x}$  and entered these vectors into the neighborhood functions  $g_i$  and  $g_j$  to generate the mean term for each pair of nodes.

## 2. Task definitions

As we describe in the main text, we assume that each agent  $i$  works to advance the team's task  $h(\vec{x})$  through their decisions  $x_i \in [0, 1]$ . Each agent receives feedback from a neighborhood function  $g_i(x_i, \vec{x}_j)$  that describes how well the agent performs on the team's task given the indirect influences of their neighbors  $j$ . We assume that agents work toward the same goal as the team and so use the same task for  $h(\vec{x})$  and each  $g_i(x_i, \vec{x}_j)$  during each simulation run of the model.

We constructed a series of tasks  $y(\vec{x}_m)$ , where  $\vec{x}_m$  is a vector of  $d$  decision variables  $x_m$  such that  $m \in M$ . Each task is scalable, normalized, and commutative. By scalable, we mean that we can describe the task  $y$  with the same equation form regardless of the number of inputs  $d$ . Consequently,  $y$  is said to be  $d$ -dimensional. This scalability is true with many optimization test functions (10), like the Ackley function (see task [ah](#)). Next, the tasks are normalized in that  $y \in [0, 1]$  regardless of the number of inputs  $d$ . Then, the tasks are commutative because the order of the inputs  $m \in M$  does not matter and any decision variable  $x_m$  can take any position in the task equation (with four exceptions, discussed later in this section). An average function of a normalized set of values is a common example of such a function that can accept any number of inputs, always returns outputs in the range of  $[0, 1]$ , and for which input order does not matter. Consequently, the functions describing each task at the team-level are functions  $h(\vec{x}) = y(\vec{x})$  composed of all agents' actions so that  $\vec{x}_m = \vec{x}$ . Then, the functions describing a task from the perspective of an agent's neighborhood are  $g_i(x_i, \vec{x}_j) = y(x_i, \vec{x}_j)$  where  $\vec{x}_m = [x_i, x_{j=1}, \dots, x_{j=J_i}]$ .

Each of the following subsections describes one of the 34 tasks that we used in our model. Where present,  $d$  is the total number of decision variables used as inputs for the task and  $k_m$  is the number of network neighbors of agent  $m$  (also called the degree). Other variables are defined in context.

Task functions that are unweighted are simple averages of the agents' values and so divided by  $d$ . Functions that are degree-weighted are weighted averages of the agents' values divided by  $\sum_m k_m + 1$  instead of  $\sum_m k_m$ . We do this primarily because it avoids dividing by zero when an agent has no interactions with other agents, as with the empty graph and some random graphs. But as described in one of the footnotes in the main work, agents technically affect themselves and so have a directed self-edge, further justifying this increase in the number of edges by  $d$  in the denominator. Functions with a uniform frequency use a consistent  $7\pi/2$ , while those with degree frequencies use  $(1 + 2k_m)\pi/2$ . Functions with uniform exponents use the degree of the first decision variable throughout the calculations, and with degree exponents use the degree of the respective agents.

Of note, the uniform exponent versions of the low-degree square high-degree root tasks (tasks [s](#) & [u](#)), and the uniform exponent versions of the high-degree root, low-degree square tasks (tasks [w](#) & [y](#)) are the exceptions to decision variable commutativity. Each of these four tasks includes a term anchored to the first index of  $\vec{x}_m$ . To counteract any biases introduced by adding tasks with a fixed term that favors either high or low degrees, these tasks are opposites of each other by design, with task [s](#) opposite [w](#), and task [u](#) opposite to [y](#). We also added a difficulty measure that accounts for the resulting divergence between agent interests which we discuss in Sec. 1.

**a. Average function (unweighted).** See Fig. [S1a](#) on page 7 for a 2-variable example where  $k_1 = 1$  and  $k_2 = 5$ .

$$y(\vec{x}_m) = \frac{1}{d} \sum_m x_m \quad [5]$$

**b. Average function (degree-weighted).** See Fig. [S1b](#) on page 7 for a 2-variable example where  $k_1 = 1$  and  $k_2 = 5$ .

$$y(\vec{x}_m) = \frac{1}{\sum_m (k_m + 1)} \sum_m (k_m + 1) x_m \quad [6]$$

**c. Average of squares function (unweighted).** See Fig. [S1c](#) on page 7 for a 2-variable example where  $k_1 = 1$  and  $k_2 = 5$ .

$$y(\vec{x}_m) = \frac{1}{d} \sum_m x_m^2 \quad [7]$$

**d. Average of squares function (degree-weighted).** See Fig. [S1d](#) on page 7 for a 2-variable example where  $k_1 = 1$  and  $k_2 = 5$ .

$$y(\vec{x}_m) = \frac{1}{\sum_m (k_m + 1)} \sum_m (k_m + 1) x_m^2 \quad [8]$$

**e. Average of square roots function (unweighted).** See Fig. [S1e](#) on page 7 for a 2-variable example where  $k_1 = 1$  and  $k_2 = 5$ .

$$y(\vec{x}_m) = \frac{1}{d} \sum_m x_m^{1/2} \quad [9]$$

**f. Average of square roots function (degree-weighted).** See Fig. [S1f](#) on page 7 for a 2-variable example where  $k_1 = 1$  and  $k_2 = 5$ .

$$y(\vec{x}_m) = \frac{1}{\sum_m (k_m + 1)} \sum_m (k_m + 1) x_m^{1/2} \quad [10]$$

110 **g. Sin<sup>2</sup>function (unweighted, uniform frequency).** See Fig. S1g on page 7 for a 2-variable example where  $k_1 = 1$  and  $k_2 = 5$ .

$$111 \quad y(\vec{x}_m) = \frac{1}{d} \sum_m \sin^2 \left( \frac{7\pi}{2} x_m \right) \quad [11]$$

112 **h. Sin<sup>2</sup>function (unweighted, degree frequency).** See Fig. S1h on page 7 for a 2-variable example where  $k_1 = 1$  and  $k_2 = 5$ .

$$113 \quad y(\vec{x}_m) = \frac{1}{d} \sum_m \sin^2 \left( \frac{(1+2k_m)\pi}{2} x_m \right) \quad [12]$$

114 **i. Sin<sup>2</sup>function (degree-weighted, uniform frequency).** See Fig. S1i on page 7 for a 2-variable example where  $k_1 = 1$  and  $k_2 = 5$ .

$$115 \quad y(\vec{x}_m) = \frac{1}{\sum_m (k_m + 1)} \sum_m (k_m + 1) \sin^2 \left( \frac{7\pi}{2} x_m \right) \quad [13]$$

116 **j. Sin<sup>2</sup>function (degree-weighted, degree frequency).** See Fig. S1j on page 7 for a 2-variable example where  $k_1 = 1$  and  $k_2 = 5$ .

$$117 \quad y(\vec{x}_m) = \frac{1}{\sum_m (k_m + 1)} \sum_m (k_m + 1) \sin^2 \left( \frac{(1+2k_m)\pi}{2} x_m \right) \quad [14]$$

118 **k. Sin<sup>2</sup>+ square function (unweighted, uniform frequency).** See Fig. S1k on page 7 for a 2-variable example where  $k_1 = 1$  and  
119  $k_2 = 5$ .

$$120 \quad y(\vec{x}_m) = \frac{1}{2d} \sum_m \sin^2 \left( \frac{7\pi}{2} x_m \right) + x_m^2 \quad [15]$$

121 **l. Sin<sup>2</sup>+ square function (unweighted, degree frequency).** See Fig. S1l on page 7 for a 2-variable example where  $k_1 = 1$  and  
122  $k_2 = 5$ .

$$123 \quad y(\vec{x}_m) = \frac{1}{2d} \sum_m \sin^2 \left( \frac{(1+2k_m)\pi}{2} x_m \right) + x_m^2 \quad [16]$$

124 **m. Sin<sup>2</sup>+ square function (degree-weighted, uniform frequency).** See Fig. S2m on page 8 for a 2-variable example where  $k_1 = 1$   
125 and  $k_2 = 5$ .

$$126 \quad y(\vec{x}_m) = \frac{1}{2 \sum_m (k_m + 1)} \sum_m (k_m + 1) \left( \sin^2 \left( \frac{7\pi}{2} x_m \right) + x_m^2 \right) \quad [17]$$

127 **n. Sin<sup>2</sup>+ square function (degree-weighted, degree frequency).** See Fig. S2n on page 8 for a 2-variable example where  $k_1 = 1$  and  
128  $k_2 = 5$ .

$$129 \quad y(\vec{x}_m) = \frac{1}{2 \sum_m (k_m + 1)} \sum_m (k_m + 1) \left( \sin^2 \left( \frac{(1+2k_m)\pi}{2} x_m \right) + x_m^2 \right) \quad [18]$$

130 **o. Sin<sup>2</sup>+ square root function (unweighted, uniform frequency).** See Fig. S2o on page 8 for a 2-variable example where  $k_1 = 1$   
131 and  $k_2 = 5$ .

$$132 \quad y(\vec{x}_m) = \frac{1}{2d} \sum_m \sin^2 \left( \frac{7\pi}{2} x_m \right) + x_m^{1/2} \quad [19]$$

133 **p. Sin<sup>2</sup>+ square root function (unweighted, degree frequency).** See Fig. S2p on page 8 for a 2-variable example where  $k_1 = 1$   
134 and  $k_2 = 5$ .

$$135 \quad y(\vec{x}_m) = \frac{1}{2d} \sum_m \sin^2 \left( \frac{(1+2k_m)\pi}{2} x_m \right) + x_m^{1/2} \quad [20]$$

136 **q. Sin<sup>2</sup>+ square root function (degree-weighted, uniform frequency).** See Fig. S2q on page 8 for a 2-variable example where  
137  $k_1 = 1$  and  $k_2 = 5$ .

$$138 \quad y(\vec{x}_m) = \frac{1}{2 \sum_m (k_m + 1)} \sum_m (k_m + 1) \left( \sin^2 \left( \frac{7\pi}{2} x_m \right) + x_m^{1/2} \right) \quad [21]$$

139 **r. Sin<sup>2</sup>+ square root function (degree-weighted, degree frequency).** See Fig. S2r on page 8 for a 2-variable example where  
140  $k_1 = 1$  and  $k_2 = 5$ .

$$141 \quad y(\vec{x}_m) = \frac{1}{2 \sum_m (k_m + 1)} \sum_m (k_m + 1) \left( \sin^2 \left( \frac{(1+2k_m)\pi}{2} x_m \right) + x_m^{1/2} \right) \quad [22]$$

142 **s. Low-degree square, high-degree root function (unweighted, uniform exponents).** Here,  $c_m = 1 - \frac{2k_1}{1 + \sum_m k_m}$ . See Fig. S2s  
 143 on page 8 for a 2-variable example where  $k_1 = 1$  and  $k_2 = 5$ .

$$144 \quad y(\vec{x}_m) = \frac{1}{d} \sum_m x_m^{2^{c_m}} \quad [23]$$

145 **t. Low-degree square, high-degree root function (unweighted, degree exponents).** Here,  $c_m = 1 - \frac{2k_m}{1 + \sum_m k_m}$ . See Fig. S2t on  
 146 page 8 for a 2-variable example where  $k_1 = 1$  and  $k_2 = 5$ .

$$147 \quad y(\vec{x}_m) = \frac{1}{d} \sum_m x_m^{2^{c_m}} \quad [24]$$

148 **u. Low-degree square, high-degree root function (degree-weighted, uniform exponents).** Here,  $c_m = 1 - \frac{2k_1}{1 + \sum_m k_m}$ . See  
 149 Fig. S2u on page 8 for a 2-variable example where  $k_1 = 1$  and  $k_2 = 5$ .

$$150 \quad y(\vec{x}_m) = \frac{1}{\sum_m (k_m + 1)} \sum_m (k_m + 1) x_m^{2^{c_m}} \quad [25]$$

151 **v. Low-degree square, high-degree root function (degree-weighted, degree exponents).** Here,  $c_m = 1 - \frac{2k_m}{1 + \sum_m k_m}$ . See Fig. S2v  
 152 on page 8 for a 2-variable example where  $k_1 = 1$  and  $k_2 = 5$ .

$$153 \quad y(\vec{x}_m) = \frac{1}{\sum_m (k_m + 1)} \sum_m (k_m + 1) x_m^{2^{c_m}} \quad [26]$$

154 **w. High-degree square, low-degree root function (unweighted, uniform exponents).** Here,  $c_m = 1 - \frac{2k_1}{1 + \sum_m k_m}$ . See Fig. S2w  
 155 on page 8 for a 2-variable example where  $k_1 = 1$  and  $k_2 = 5$ .

$$156 \quad y(\vec{x}_m) = \frac{1}{d} \sum_m x_m^{2^{-c_m}} \quad [27]$$

157 **x. High-degree square, low-degree root function (unweighted, degree exponents).** Here,  $c_m = 1 - \frac{2k_m}{1 + \sum_m k_m}$ . See Fig. S2x on  
 158 page 8 for a 2-variable example where  $k_1 = 1$  and  $k_2 = 5$ .

$$159 \quad y(\vec{x}_m) = \frac{1}{d} \sum_m x_m^{2^{-c_m}} \quad [28]$$

160 **y. High-degree square, low-degree root function (degree-weighted, uniform exponents).** Here,  $c_m = 1 - \frac{2k_1}{1 + \sum_m k_m}$ . See  
 161 Fig. S3y on page 9 for a 2-variable example where  $k_1 = 1$  and  $k_2 = 5$ .

$$162 \quad y(\vec{x}_m) = \frac{1}{\sum_m (k_m + 1)} \sum_m (k_m + 1) x_m^{2^{-c_m}} \quad [29]$$

163 **z. High-degree square, low-degree root function (degree-weighted, degree exponents).** Here,  $c_m = 1 - \frac{2k_m}{1 + \sum_m k_m}$ . See Fig. S3z  
 164 on page 9 for a 2-variable example where  $k_1 = 1$  and  $k_2 = 5$ .

$$165 \quad y(\vec{x}_m) = \frac{1}{\sum_m (k_m + 1)} \sum_m (k_m + 1) x_m^{2^{-c_m}} \quad [30]$$

166 **aa. Maximum function.** See Fig. S3aa on page 9 for a 2-variable example where  $k_1 = 1$  and  $k_2 = 5$ .

$$167 \quad y(\vec{x}_m) = \max(x_m) \quad [31]$$

168 **ab. Minimum function.** See Fig. S3ab on page 9 for a 2-variable example where  $k_1 = 1$  and  $k_2 = 5$ .

$$169 \quad y(\vec{x}_m) = \min(x_m) \quad [32]$$

170 **ac. Median function.** See Fig. S3ac on page 9 for a 2-variable example where  $k_1 = 1$  and  $k_2 = 5$ .

$$171 \quad y(\vec{x}_m) = \text{median}(x_m) \quad [33]$$

172 **ad.  $K + 1$  power function (unweighted).** See Fig. S3ad on page 9 for a 2-variable example where  $k_1 = 1$  and  $k_2 = 5$ .

$$173 \quad y(\vec{x}_m) = \frac{1}{d} \sum_m x_m^{k_m+1} \quad [34]$$

174 **ae.  $K + 1$  power function (degree-weighted).** See Fig. S3ae on page 9 for a 2-variable example where  $k_1 = 1$  and  $k_2 = 5$ .

$$175 \quad y(\vec{x}_m) = \frac{1}{\sum_m (k_m + 1)} \sum_m (k_m + 1) x_m^{k_m+1} \quad [35]$$

176 **af.  $K + 1$  Root function (unweighted).** See Fig. S3af on page 9 for a 2-variable example where  $k_1 = 1$  and  $k_2 = 5$ .

$$177 \quad y(\vec{x}_m) = \frac{1}{d} \sum_m x_m^{\frac{1}{k_m+1}} \quad [36]$$

178 **ag.  $K + 1$  Root function (degree-weighted).** See Fig. S3ag on page 9 for a 2-variable example where  $k_1 = 1$  and  $k_2 = 5$ .

$$179 \quad y(\vec{x}_m) = \frac{1}{\sum_m (k_m + 1)} \sum_m (k_m + 1) x_m^{\frac{1}{k_m+1}} \quad [37]$$

180 **ah. Ackley function.** For this implementation, we invert the Ackley function from its traditional concave form (for minimizing)  
 181 to a convex form (for maximizing). Here,  $c_1 = 20$ ,  $c_2 = 0.2$ , and  $c_3 = 7\pi$ . See Fig. S3ah on page 9 for a 2-variable example  
 182 where  $k_1 = 1$  and  $k_2 = 5$ .

$$183 \quad y(\vec{x}_m) = 1 - \frac{-c_1 \exp\left(-c_2 \sqrt{\frac{1}{k_i+1} \sum_m x_m^2}\right) - \exp\left(\frac{1}{k_i+1} \sum_m \cos(c_3 x_m)\right) + \exp(1) + c_1}{c_1 (1 - \exp(-c_2)) + (\exp(1) - \exp(-1))} \quad [38]$$

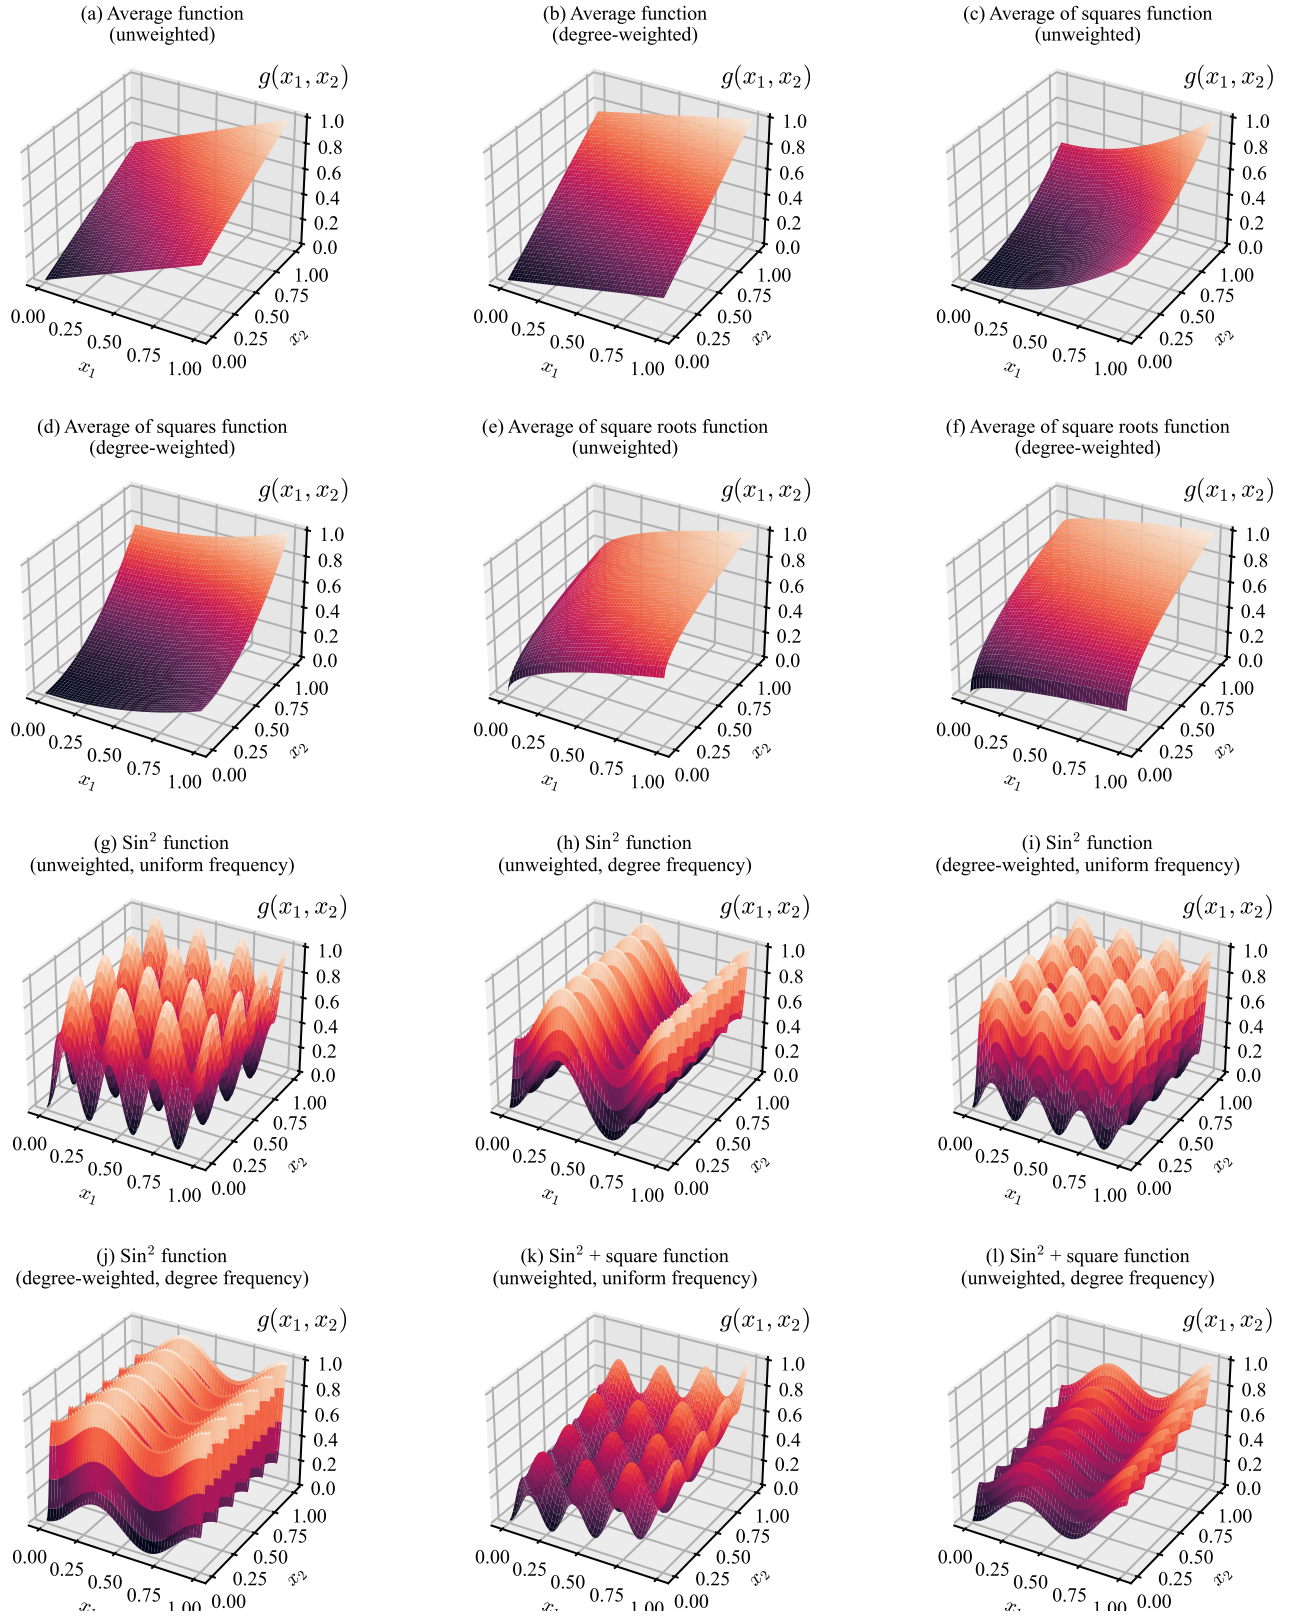

Fig. S1. Tasks (a-l).

(m)  $\text{Sin}^2$  + square function  
(degree-weighted, uniform frequency)

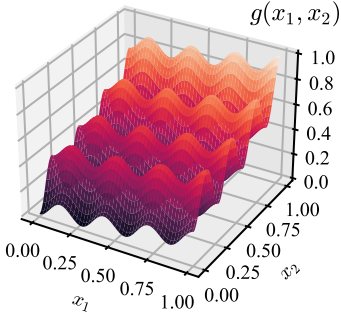

(n)  $\text{Sin}^2$  + square function  
(degree-weighted, degree frequency)

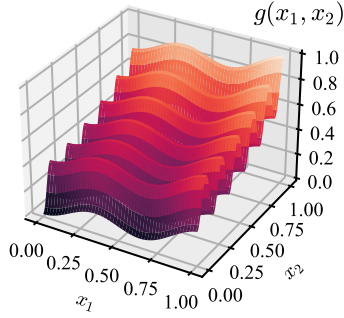

(o)  $\text{Sin}^2$  + square root function  
(unweighted, uniform frequency)

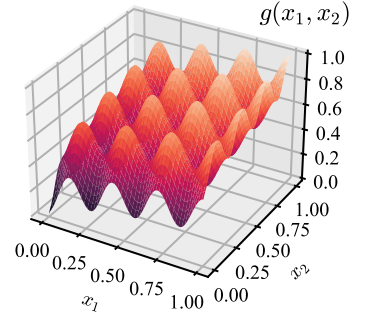

(p)  $\text{Sin}^2$  + square root function  
(unweighted, degree frequency)

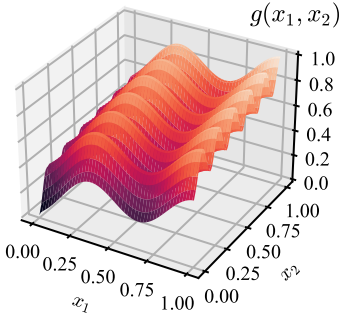

(q)  $\text{Sin}^2$  + square root function  
(degree-weighted, uniform frequency)

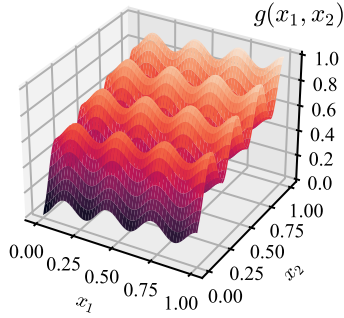

(r)  $\text{Sin}^2$  + square root function  
(degree-weighted, degree frequency)

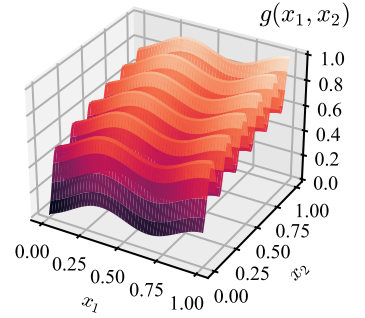

(s) Low-degree square, high-degree root function  
(unweighted, uniform exponents)

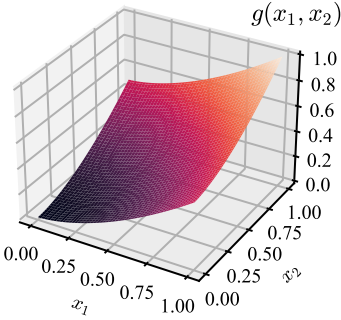

(t) Low-degree square, high-degree root function  
(unweighted, degree exponents)

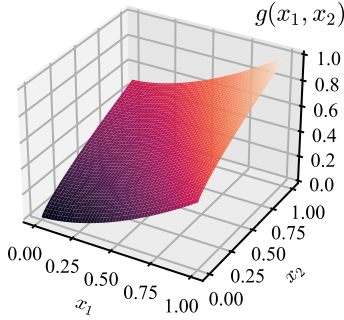

(u) Low-degree square, high-degree root function  
(degree-weighted, uniform exponents)

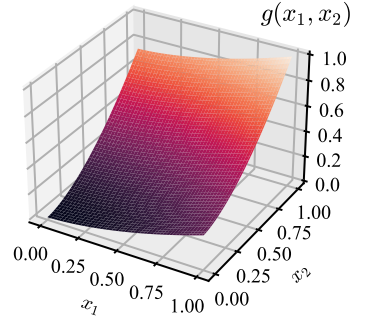

(v) Low-degree square, high-degree root function  
(degree-weighted, degree exponents)

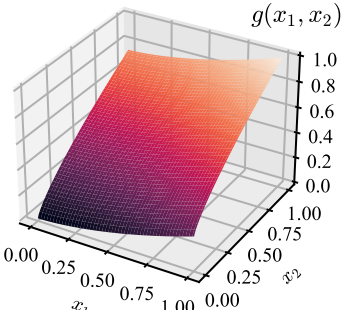

(w) High-degree square, low-degree root function  
(unweighted, uniform exponents)

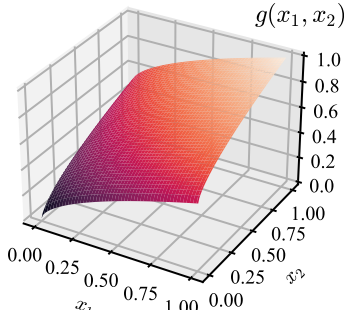

(x) High-degree square, low-degree root function  
(unweighted, degree exponents)

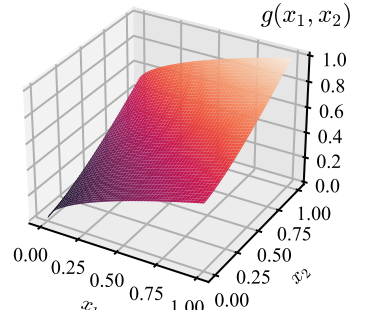

Fig. S2. Tasks (m-x).

(y) High-degree square, low-degree root function  
(degree-weighted, uniform exponents)

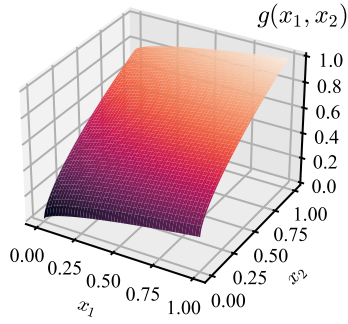

(z) High-degree square, low-degree root function  
(degree-weighted, degree exponents)

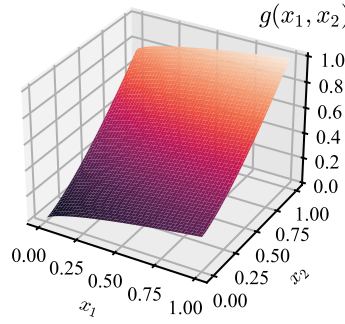

(aa) Maximum function

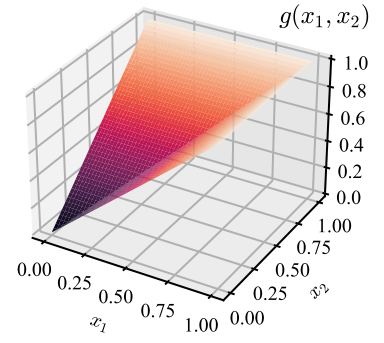

(ab) Minimum function

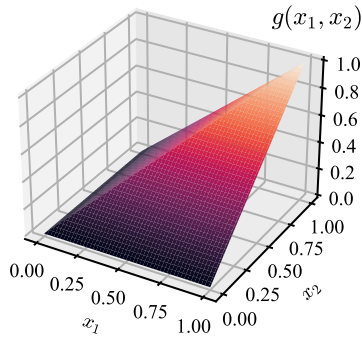

(ac) Median function

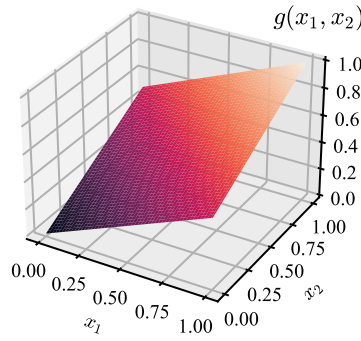

(ad) K+1 power function  
(unweighted)

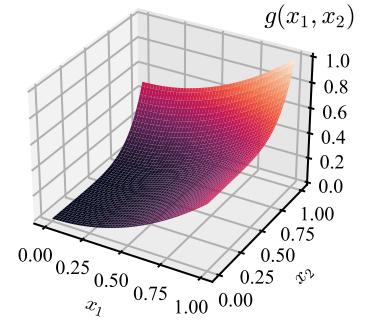

(ae) K+1 power function  
(degree-weighted)

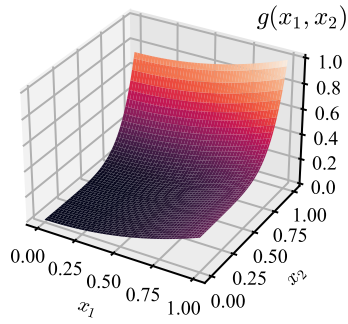

(af) K+1 Root function  
(unweighted)

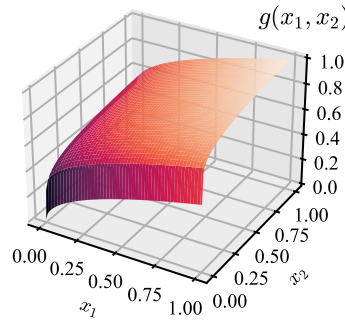

(ag) K+1 Root function  
(degree-weighted)

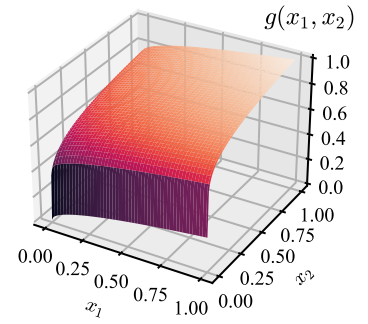

(ah) Ackley function

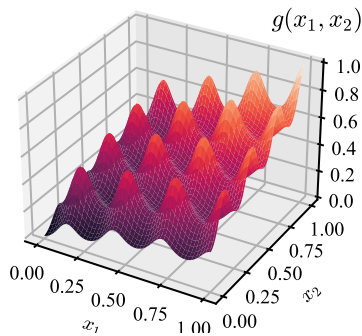

Fig. S3. Tasks (y-ah).

### 3. Network measures

We measured common properties of network structure (11) for each team using algorithms provided by the python package NetworkX (12). Degree centrality (mean and standard deviation) measures how connected individuals are to one another (11). Next, eigenvector centrality and nearest neighbor degree (mean and standard deviation of each) measure how connected individuals are to individuals who are themselves highly-connected (11). For eigenvector centrality specifically, high means indicate evenly distributed connectedness and decentralized networks, while high standard deviations indicate varied connectedness and centralization. The mean of the shortest path length, betweenness centrality (mean and standard deviation), and diameter measure how efficiently information can flow from each node to each other node. And last, the clustering coefficient and assortativity measure how often individuals are connected to the same individuals.

Below, we specify the NetworkX algorithm we used and any details for each measure and group them by aspects of the network that they measure. We used each algorithm's default values unless otherwise specified. Averages and standard deviations were calculated by taking the mean and standard deviation over all nodes in the team for that run of the model. All measures are valid for any network except assortativity, shortest path length, and diameter, which are only defined on completely connected graphs.

- Measures of individual connectedness
  - Degree centrality (mean and standard deviation)
    - \* Mean describes how well-connected individuals are on average
    - \* Standard deviation describes how much variation there is in individuals' connectedness
    - \* Measured with `algorithms.centrality.degree_centrality`
    - \* Valid on connected and disconnected graphs
- Measures of neighbors' connectedness
  - Eigenvector centrality (mean and standard deviation)
    - \* Describes how centralized a network is (13)
    - \* Mean eigenvector centrality describes how decentralized a network is because higher mean values indicate that most or all individuals are nearly as important as one another.
    - \* Higher standard deviations represents how centralized a network is because higher values correspond to a fewer individuals holding more importance than most others
    - \* Measured with `algorithms.centrality.eigenvector_centrality` (tolerance: 0.001, max iterations: 1000)
    - \* Valid on connected and disconnected graphs
  - Nearest neighbor degree (mean and standard deviation)
    - \* Mean describes how well-connected an individual's neighbors are on average
    - \* Standard deviation describes how much variation there is in how well-connected an individual's neighbors are
    - \* Measured with `algorithms.assortativity.average_neighbor_degree`
    - \* Valid on connected and disconnected graphs
- Measures of network efficiency
  - Betweenness centrality (mean and standard deviation)
    - \* Mean indicates how often individuals are intermediaries on the shortest path between two individuals
    - \* Standard deviation indicates variation in the number of intermediaries between individuals in the network
    - \* Measured with `algorithms.centrality.betweenness_centrality`
    - \* Valid on connected and disconnected graphs
  - Shortest path length
    - \* Measured with `algorithms.shortest_paths.generic.average_shortest_path_length`
    - \* Only valid on connected graphs
  - Diameter
    - \* Measured with `algorithms.distance_measures.diameter`
    - \* Only valid on connected graphs
- Measures of shared connections
  - Degree assortativity
    - \* Measured with `algorithms.assortativity.degree_assortativity_coefficient`
    - \* Only valid on connected graphs
  - Clustering coefficient
    - \* Measured with `algorithms.cluster.average_clustering`
    - \* Valid on connected and disconnected graphs

## 4. Network definitions

In this work, we constructed 12 different types of networks (three of which included probabilistic variants) of four different sizes,  $n \in \{4, 9, 16, 25\}$ . To select networks to include in this study, we began by compiling a list of networks widely used in previous works on teams and organizations. These included the complete graph, the empty graph, preferential attachment graphs, random graphs, small world graphs, the star graph, the tree graph, and the ring of cliques (6–8, 14–17). To introduce greater variation in network properties, we supplemented this list with networks provided in the python package NetworkX (12) and suggested by colleagues, adding the ring graph, the rook’s graph, the wheel graph, and the windmill graph. Below, we briefly describe the constructions of these networks. See Fig. S4 on page 12 for a graphical representation of each network and each size team.

**Complete graph.** A network in which every node is connected to every other node.

**Empty graph.** A network in which no nodes are connected to any other nodes. In this work, an empty graph represents individual learning.

**Random graph.** A randomly-generated network in which a probability  $p$  specifies the likelihood that an edge exists between any two nodes.

**Ring graph.** A network in which each node is connected to two other nodes in a cycle, roughly forming the shape of a ring for large  $n$ .

**Small world graph.** A ring network in which each node is connected to its  $k$  nearest neighbors. Then, each edge is rewired to another random node with probability  $p$ . For our study, we created small world graphs of  $k = 2$ , but with three different probabilities of rewiring  $p \in \{0.1, 0.5, 0.9\}$ .

**Preferential attachment graph.** A preferential attachment network generated using the Holme-Kim algorithm (18). This algorithm places new nodes  $i$  in the graph, and connects each  $i$  to existing nodes  $j$  by placing  $m$  edges following traditional preferential attachment. Then, for each neighbor  $j$ , there is a probability  $p$  that  $i$  will be connected to one of  $j$ ’s neighbors by adding a new edge to form a triangle. For this work, we used  $m = 2$  and  $p \in \{0.1, 0.5, 0.9\}$ .

**Ring of cliques graph.** This network is a set of completely-connected groups or “cliques” where two members of each clique have an additional edge connecting them to another clique. The cliques are connected in a ring-like pattern. Our implementation places  $\sqrt{n}$  nodes in each of  $\sqrt{n}$  cliques for each team size  $n$ , which partially motivated our selection of the values of  $n$  we used. At  $n = 4$ , the ring of cliques is identical to a ring graph with  $n = 4$ , but the distinction becomes meaningful thereafter. Teams of  $n = 9$  produce 3 connected cliques of 3;  $n = 16$  produces 4 cliques of 4, and  $n = 25$  produces 5 cliques of 5.

**Rook’s graph.** A network in which nodes are placed in a square grid. Every node is connected to every other node in its column with an edge, and likewise every node is connected to every other node in its row with an edge. Traditionally, each node metaphorically represents a location on a chess board and each edge represents the possible moves that a rook could make from each position on the board, though the board can be of arbitrary size (19). In this work, we created rook’s graphs for each value of  $n$  where the length of each side is  $\sqrt{n}$ , corresponding to teams placed in  $2 \times 2$  grids (again, a simple ring),  $3 \times 3$  grids,  $4 \times 4$  grids, and a  $5 \times 5$  grids, again with every node connected to all other nodes in their same row and column.

**Star graph.** A network of  $n$  nodes in which  $n - 1$  nodes are each connected to one central node, and only to that central node.

**Tree graph.** A network in which new nodes are randomly connected to an existing node when placed, creating a source and “branches” or “roots.”

**Wheel graph.** This network is a combination of both the ring graph and a star graph. One central node is connected to  $n - 1$  nodes, and those  $n - 1$  nodes are connected to one another in a ring.

**Windmill graph.** A network in which  $c$  completely-connected cliques, each of  $k$  nodes, are all connected to one another via one node which is a member of every clique. This creates an effect where networks look like sails connected to a shaft, like a windmill. We constructed windmills of  $c = \sqrt{n} + 1$  cliques where each clique has  $k = \sqrt{n}$  nodes. This created teams of  $n = 4$  with 3 cliques of 2 nodes;  $n = 9$  with 4 cliques of 3 nodes;  $n = 16$  with 5 cliques of 4 nodes; and  $n = 25$  with 6 cliques of 5 nodes.

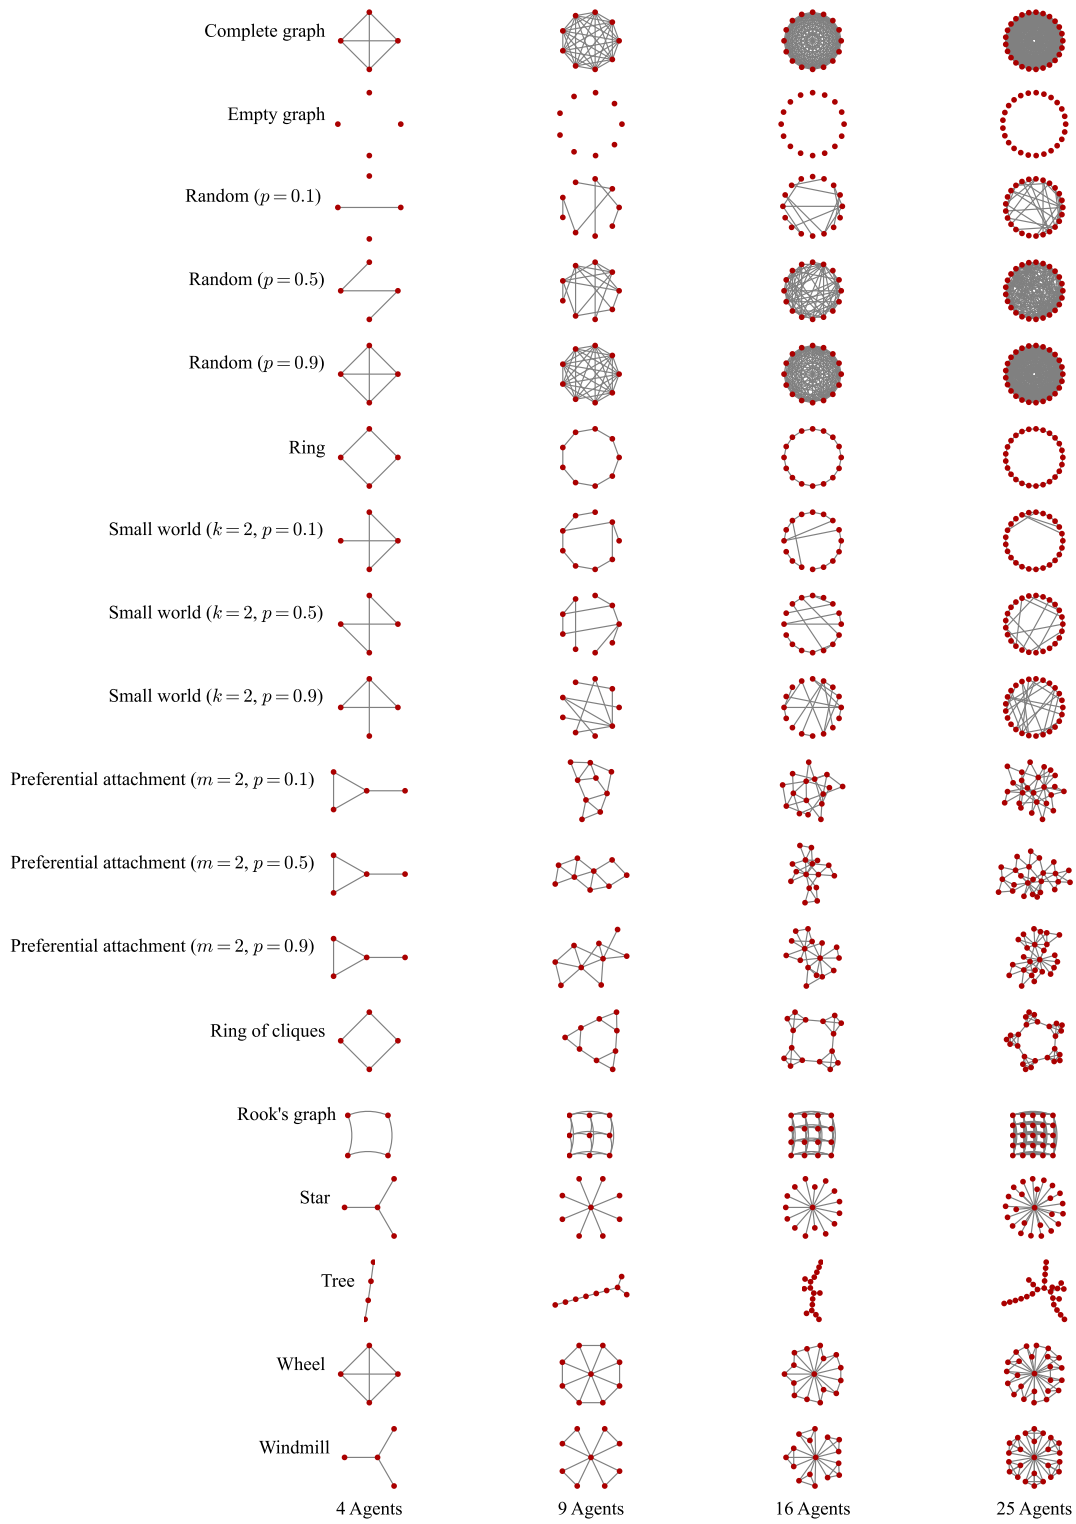

**Fig. S4.** Networks for each team size used in the model.

## 283 5. Performance by task and network

284 The heatmaps and bar graphs in Figs. S5-S8 (pages 14-17) show performance results for teams of  $n = 9$  agents. Each figure  
285 shows results for one search radius  $r$ . Within each figure, the heatmap shows the performance of teams with each network  
286 on each task, averaged over all 250 runs and all timesteps. The top bar graphs shows the mean and standard deviation of  
287 team performance for each network type compared to the performance averaged over all networks (with the same number of  
288 agents and the same search radius). The right bars show the mean and standard deviation of team performance for each task  
289 compared to the performance averaged over all tasks.

## 290 6. Average performances by network and search radius

291 As with the average performance figure in the main text, Fig. S9 contains the average performance of teams of  $n \in \{4, 9, 16, 25\}$ .  
292 The figures corroborate that dense teams tend to perform better on local “exploitation” searches while sparse teams tend to  
293 perform better on global “exploration” searches. This trend is less clear for small teams ( $n = 4$ ), but network structures are  
294 less distinct from one another at this scale (see Fig. S4 for examples). Otherwise, the trend appears to hold across sizes. Here,  
295 we also include results for  $r = 0.001$ . This radius is much smaller than the smallest feature of any task and so functionally acts  
296 as a random starting point with slight perturbations. As expected, this search radius yielded random results for small teams,  
297 and mirrored the results of  $r = 0.01$  for larger teams where the greater potential of interaction gradually increases the odds of  
298 affecting performance.

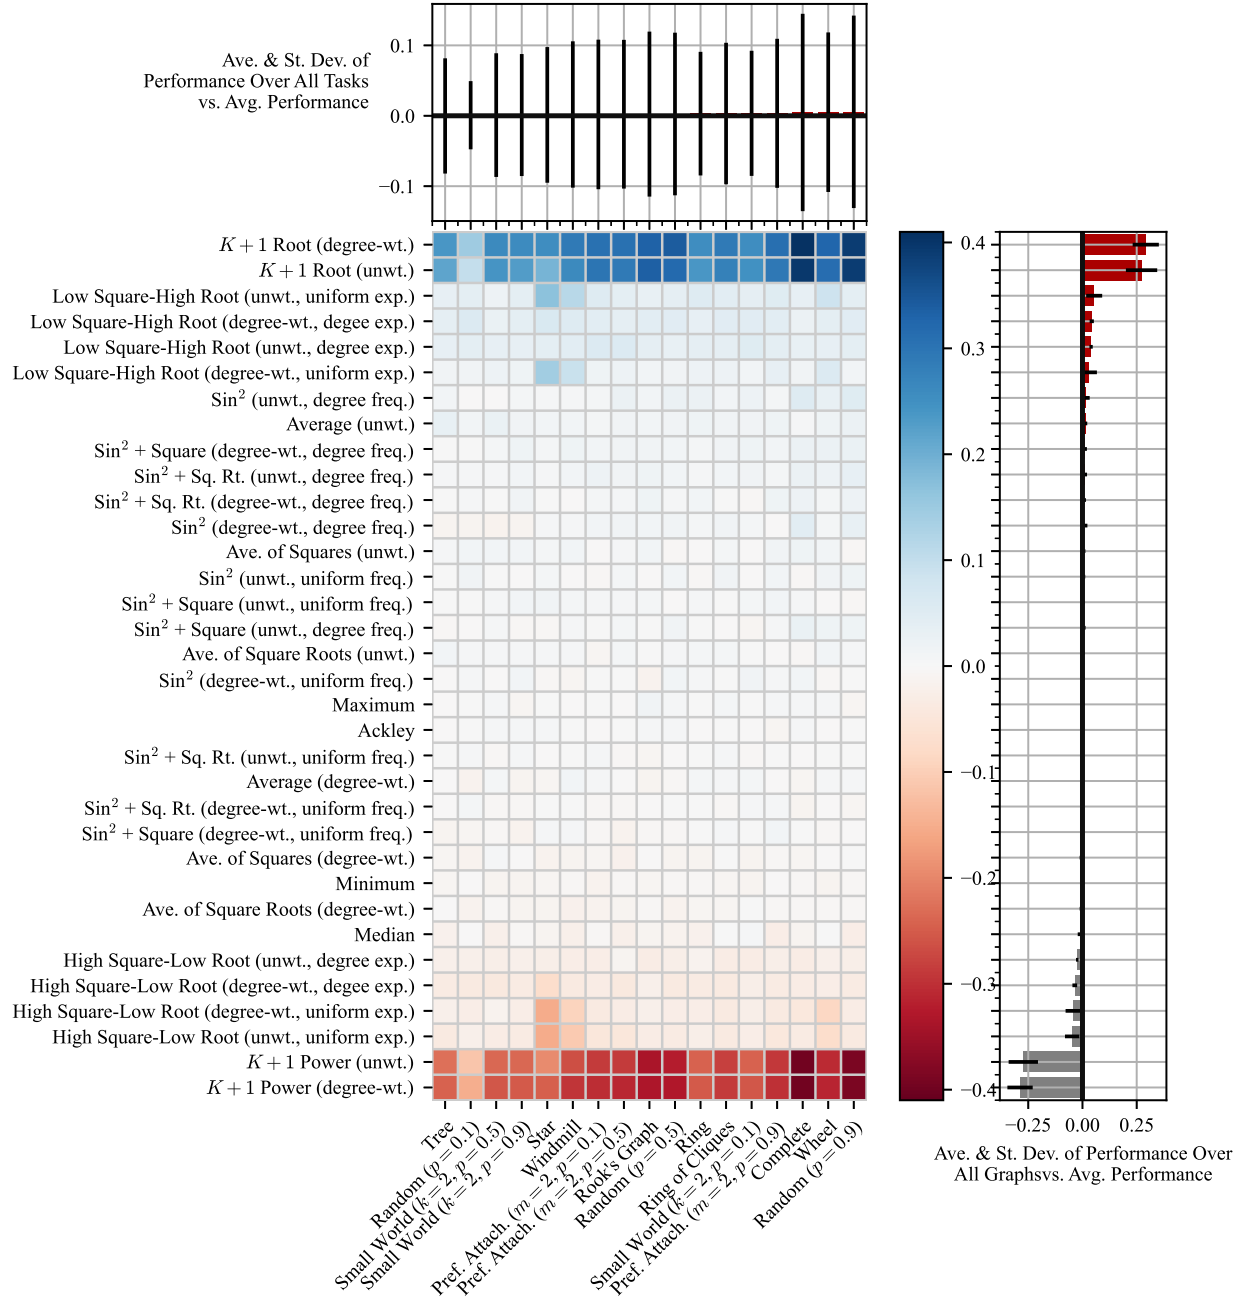

**Fig. S5. Network task performance, teams of  $n = 9$ , search radius of  $r = 0.001$ .** (Center) A heatmap of the average performance, with one column for each network and one row for each task, after subtracting the team performance of the empty graph (individual learning case) on that task. (Top) Average performance of each network across all tasks with one standard deviation, after subtracting the average performance across all networks. (Right) Average performance on each task across all networks with one standard deviation, after subtracting the average performance across all tasks.

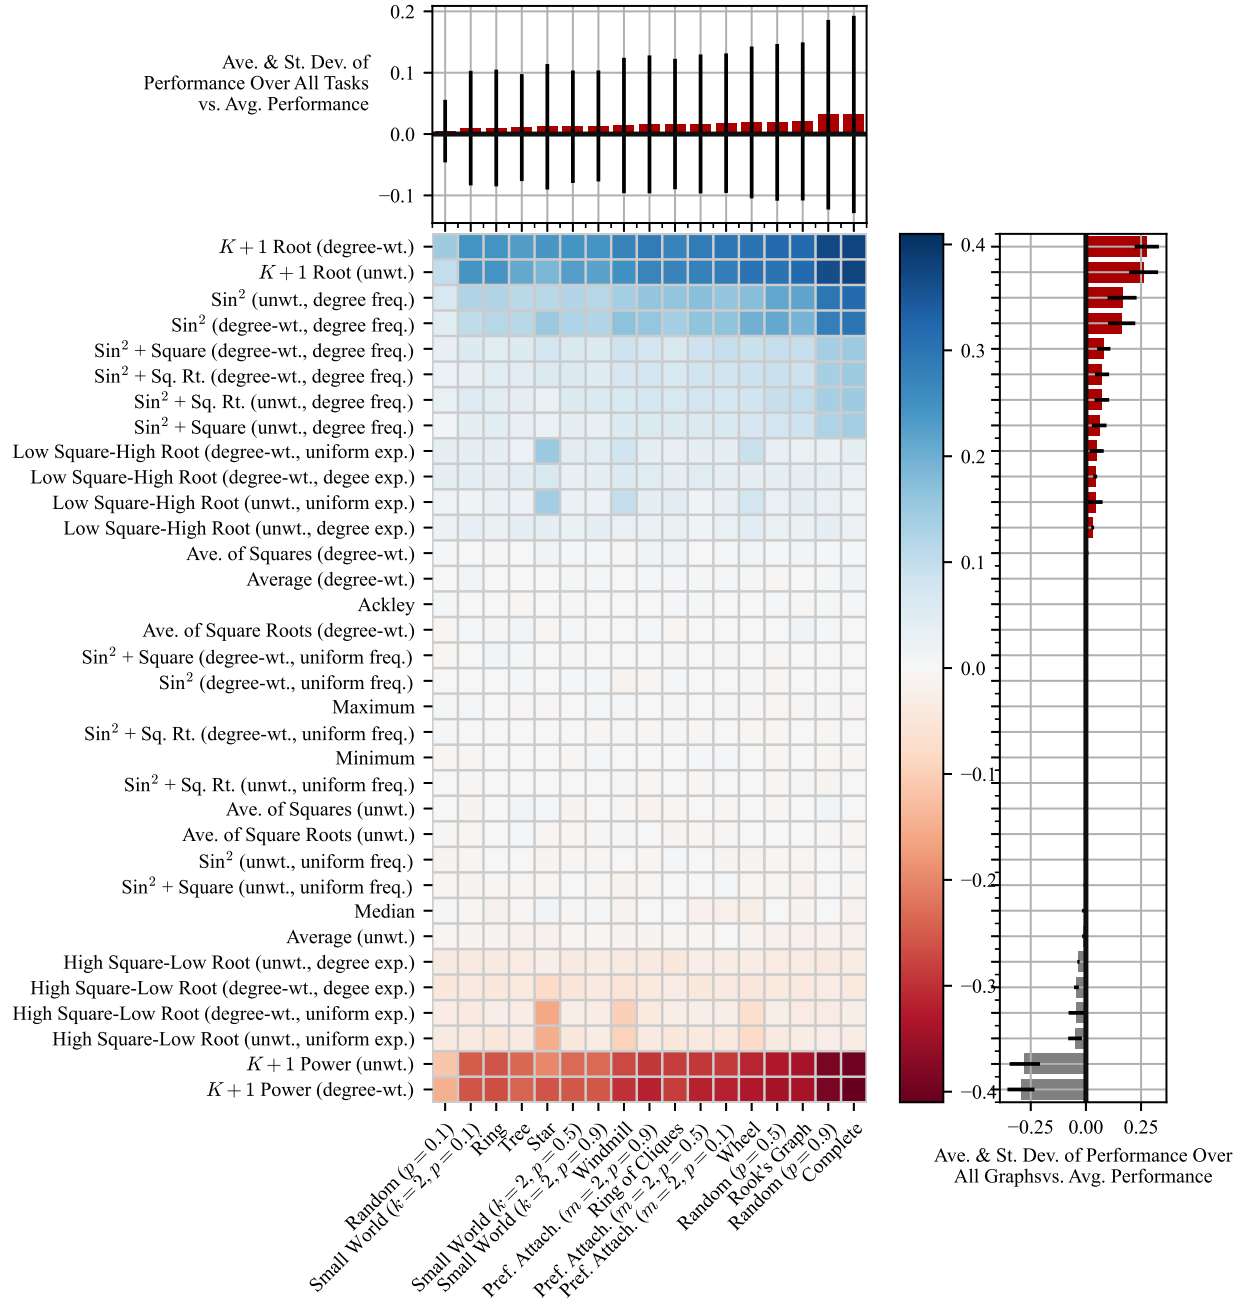

**Fig. S6. Network task performance, teams of  $n = 9$ , search radius of  $r = 0.01$ .** (Center) A heatmap of the average performance, with one column for each network and one row for each task, after subtracting the team performance of the empty graph (individual learning case) on that task. (Top) Average performance of each network across all tasks with one standard deviation, after subtracting the average performance across all networks. (Right) Average performance on each task across all networks with one standard deviation, after subtracting the average performance across all tasks.

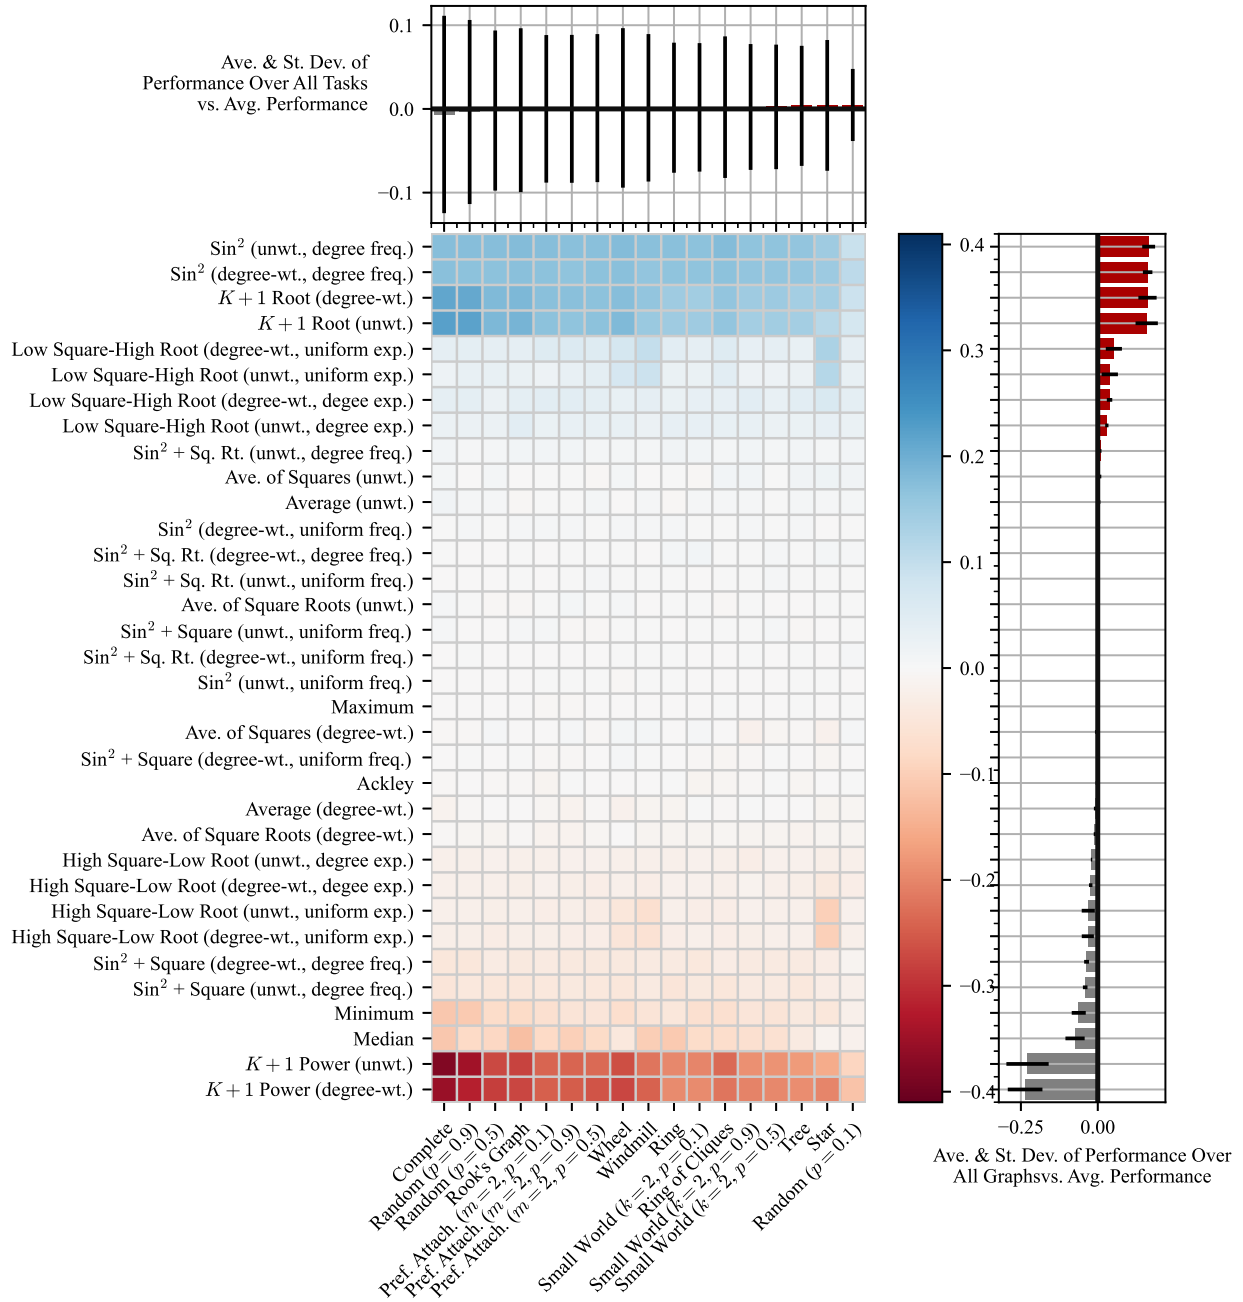

**Fig. S7. Network task performance, teams of  $n = 9$ , search radius of  $r = 0.1$ .** (Center) A heatmap of the average performance, with one column for each network and one row for each task, after subtracting the team performance of the empty graph (individual learning case) on that task. (Top) Average performance of each network across all tasks with one standard deviation, after subtracting the average performance across all networks. (Right) Average performance on each task across all networks with one standard deviation, after subtracting the average performance across all tasks.

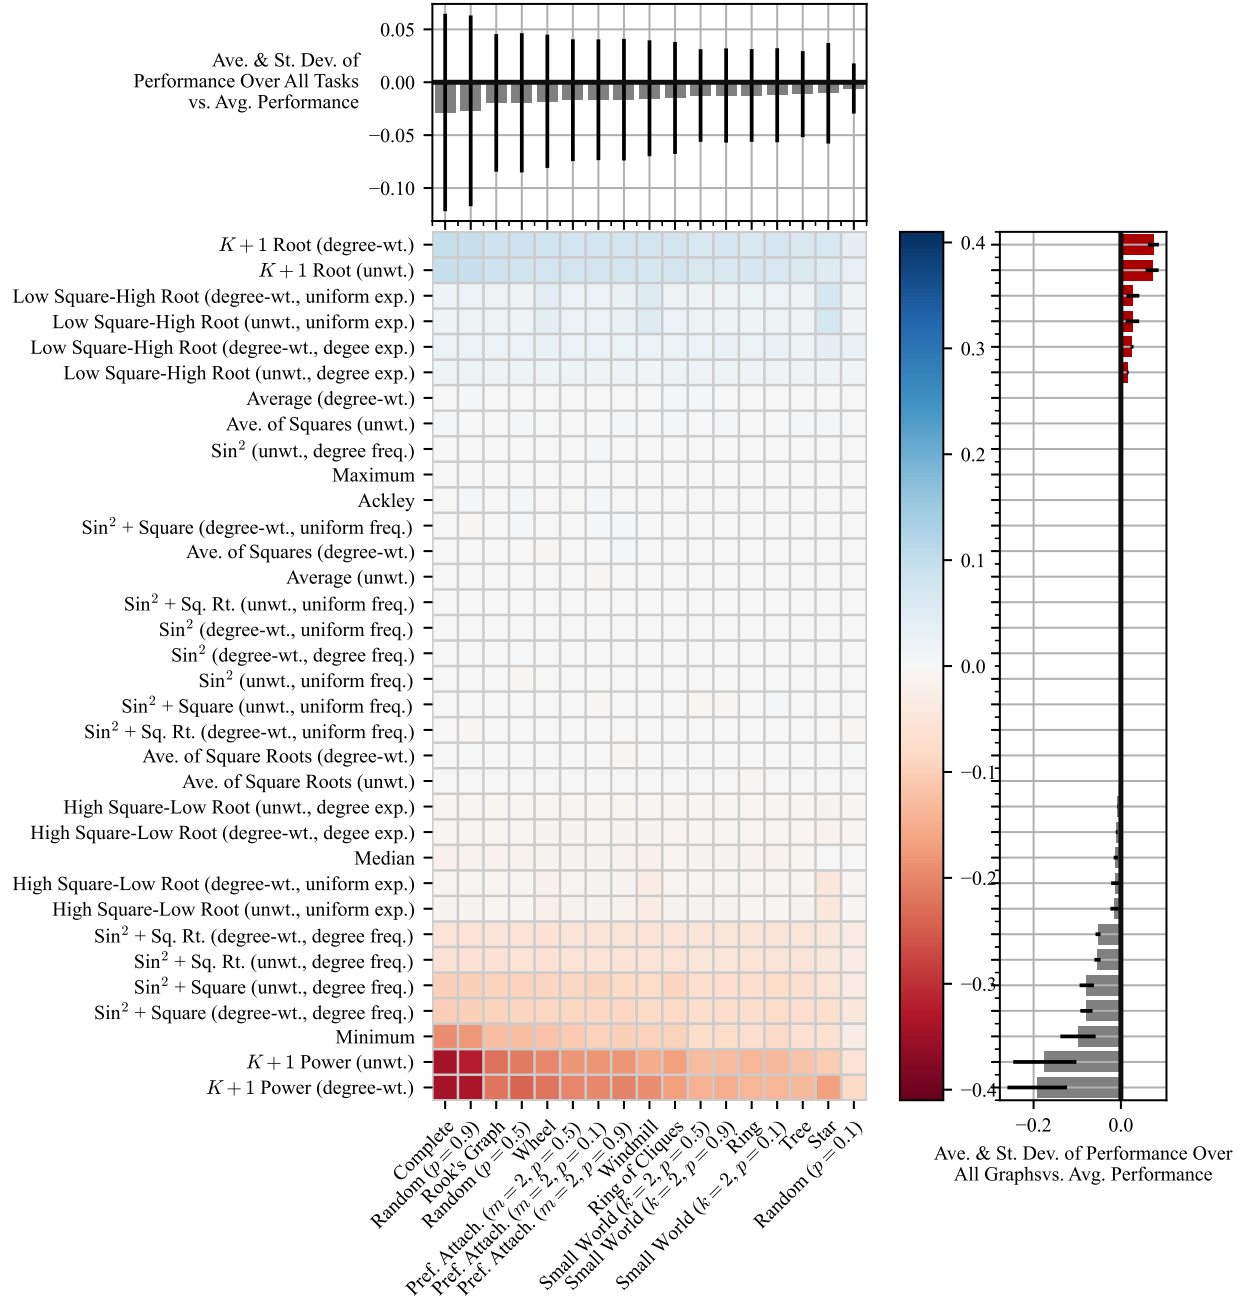

**Fig. S8. Network task performance, teams of  $n = 9$ , search radius of  $r = 1.0$ .** (Center) A heatmap of the average performance, with one column for each network and one row for each task, after subtracting the team performance of the empty graph (individual learning case) on that task. (Top) Average performance of each network across all tasks with one standard deviation, after subtracting the average performance across all networks. (Right) Average performance on each task across all networks with one standard deviation, after subtracting the average performance across all tasks.

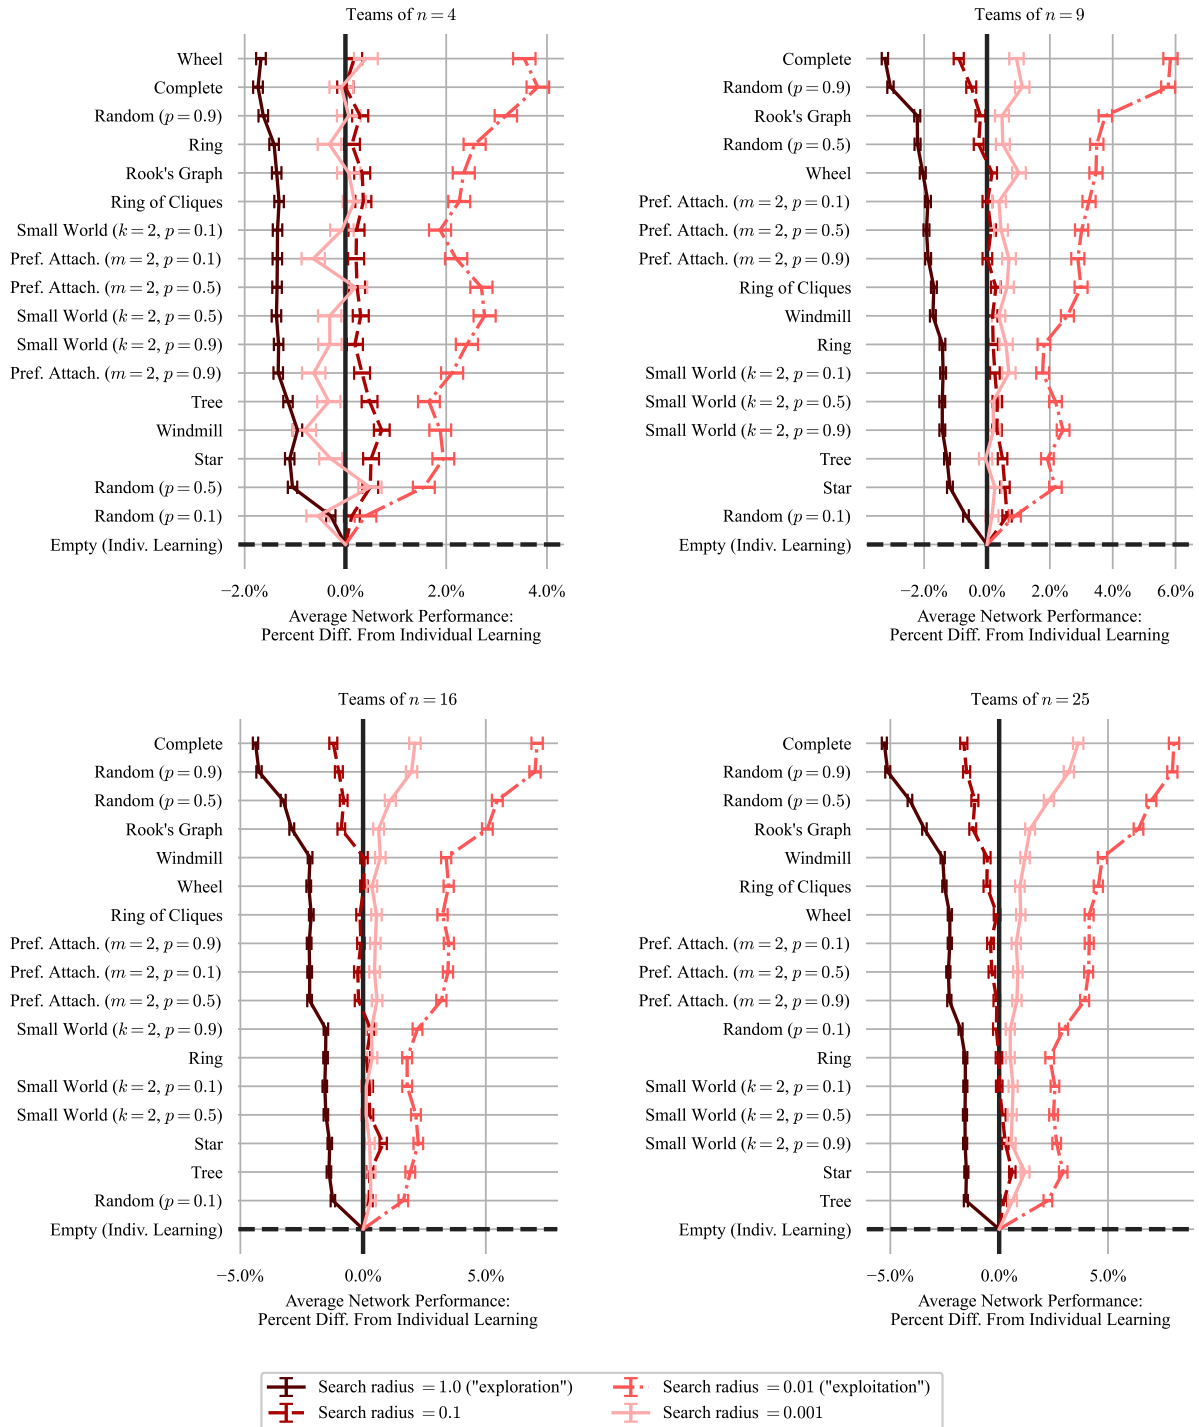

Fig. S9. The relative average performances compared to an empty graph baseline for networks of  $n \in \{4, 9, 16, 25\}$ .

## 7. Random forest analysis details

We conducted two random forest regression analyses using `ensemble.RandomForestRegressor` from Scikit-learn (20) with the default parameters. One random forest included completely-connected networks and all network measures, and the other included all networks and network measures that are still valid on disconnected graphs.

We measured the contribution of the task measures defined in Sec. 1 and included a fixed effect variable for each task. Then, we normalized each of the 12 network measures described in Sec. 3 to the range  $[0, 1]$ . We added one variable for each measure to estimate how much different qualities affect performance. The random forests also measured the effects of several control variables. We measured team progress over time through a variable for the time step of each run. Then, while the tasks themselves mostly control for team size through their normalized ranges, we added a variable for team size to control for any additional effects (which were negligible in both random forests). We also included a variable for the search radius to control for exploration abilities not attributable to network properties.

See Fig. S10 on page 20 and Tab. S1 on page 21 for the results of each.

## 8. Regression analysis details

We estimated the effects that different task and network measures have on team performance through multivariate ordinary least squares (OLS) regressions. Many of these measures are correlated (Fig. S11 on 22), a known challenge in networks research (21). We overcame this by performing six regressions with different controls. We performed three regressions using only completely-connected networks and all network measures (Tab. S2 on 23), and another three with all networks and network measures that are still valid on disconnected graphs (Tab. S3 on page 24). Within each set of three, we ran one regression with only task measures, one with only task fixed effects (that is, with  $w - 1 = 33$  dummy variables for the  $w = 34$  tasks), and one with both task measures and task fixed effects.

For these regressions, we used the python package Statsmodels (22). Each regression used robust standard errors (type HC2). We controlled for team progress over time through a variable for the  $\log_{10}$  of the time step of each run, adding one to the time step to avoid the undefined value at  $t = 0$ . Then, while the tasks themselves mostly control for team size through their normalizations, we added variables for team size and the square of team size to ensure we controlled for any additional effects (which were negligible in all regressions). We included a variable for the  $\log_{10}$  of the search radius to control for exploration abilities not attributable to network properties. The regressions included all four search radii for thoroughness.

After including these controls, we normalized each of the 12 network measures described in Sec. 3 to the range  $[0, 1]$ . We added one variable for each measure to estimate how much different qualities affect performance (as described in the Results section of the main text). In preliminary regressions, we included dummy variables for the different search radii. However, the statistically significant network measures varied approximately linearly with the  $\log_{10}$  of the search radius. Consequently, the regressions we show here included one interaction term between each measure and the  $\log_{10}$  of the search radius to measure how much the search radius (and exploration-exploitation) moderates the effect of each network measure on performance.

## 9. Network statistics

Tab. S4 on page 25 displays the average value of each network measure for each type of network used in our study for teams of  $n = 9$  individuals.

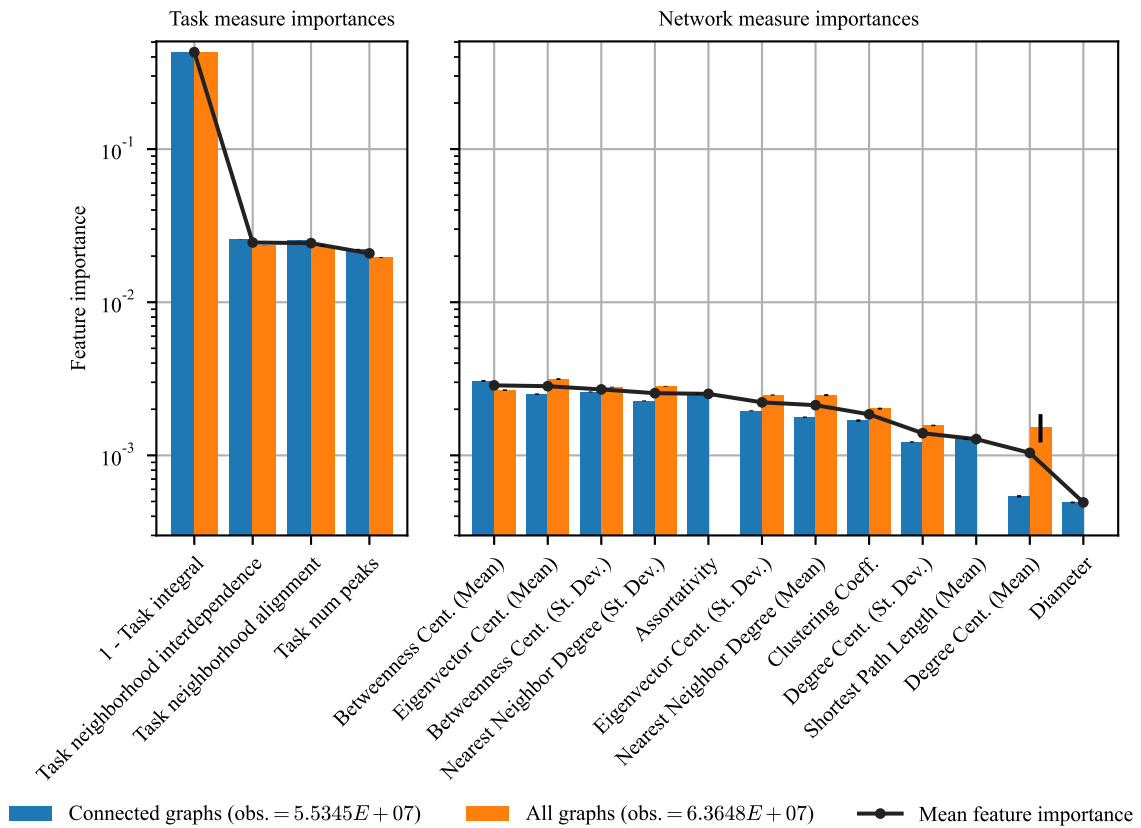

**Fig. S10. Random forest feature importances.** Error bars display the range of one standard deviation. The most important measures for team performance were the task difficulty measures. This was followed by the inefficiency of the network (measured by the mean and standard deviation of betweenness centrality) which is within one standard deviation of decentralization (measured by mean eigenvector centrality), then by variation in the connectedness of one's neighbors (via the standard deviation of nearest neighbor degree), and shared connections with neighbors (assortativity).

|                         | Observations                               | Connected graphs<br>55,342,898 | All graphs<br>63,648,000 |
|-------------------------|--------------------------------------------|--------------------------------|--------------------------|
| <b>Controls</b>         | Time step                                  | 0.104252 (0.000075)            | 0.105389 (0.000070)      |
|                         | Team size                                  | 0.000354 (0.000020)            | 0.000752 (0.000069)      |
|                         | Search radius                              | 0.361612 (0.000096)            | 0.369159 (0.000092)      |
| <b>Task measures</b>    | Exploration difficulty (1 - Task integral) | 0.432379 (0.000146)            | 0.427343 (0.000133)      |
|                         | Exploitation difficulty (Number of peaks)  | 0.022157 (0.000162)            | 0.019545 (0.000118)      |
|                         | Neighborhood alignment                     | 0.025309 (0.000061)            | 0.023335 (0.000302)      |
|                         | Neighborhood interdependence               | 0.025691 (0.000056)            | 0.023416 (0.000044)      |
| <b>Network measures</b> | Degree Cent. (Mean)                        | 0.000540 (0.000009)            | 0.001536 (0.000322)      |
|                         | Degree Cent. (St. Dev.)                    | 0.001223 (0.000013)            | 0.001569 (0.000017)      |
|                         | Eigenvector Cent. (Mean)                   | 0.002512 (0.000028)            | 0.003149 (0.000043)      |
|                         | Eigenvector Cent. (St. Dev.)               | 0.001959 (0.000013)            | 0.002480 (0.000021)      |
|                         | Betweenness Cent. (Mean)                   | 0.003067 (0.000041)            | 0.002665 (0.000033)      |
|                         | Betweenness Cent. (St. Dev.)               | 0.002599 (0.000018)            | 0.002793 (0.000017)      |
|                         | Nearest Neighbor Degree (Mean)             | 0.001779 (0.000015)            | 0.002476 (0.000038)      |
|                         | Nearest Neighbor Degree (St. Dev.)         | 0.002269 (0.000016)            | 0.002827 (0.000016)      |
|                         | Clustering Coeff.                          | 0.001688 (0.000032)            | 0.002020 (0.000029)      |
|                         | Degree Assortativity                       | 0.002522 (0.000016)            |                          |
|                         | Shortest Path Length (Mean)                | 0.001277 (0.000013)            |                          |
|                         | Diameter                                   | 0.000493 (0.000006)            |                          |

Table S1. Random forest feature importances with connected graphs and all graphs. Parenthetical values are standard deviations.

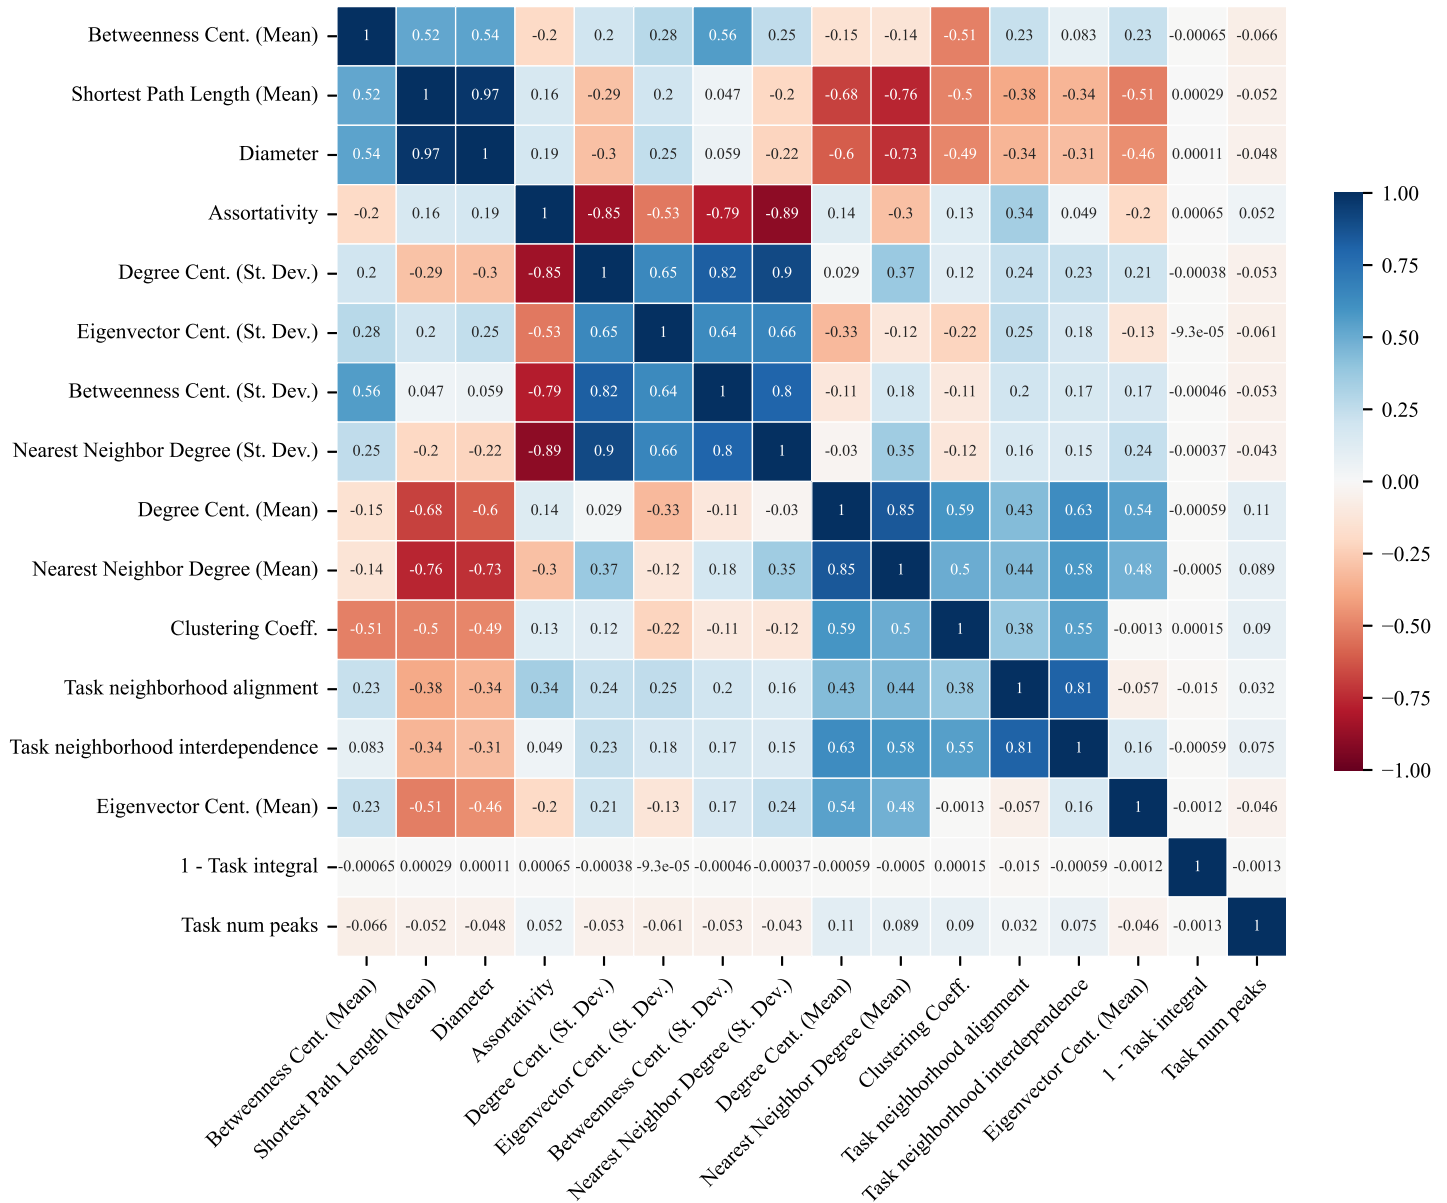

Fig. S11. Correlation coefficients for each combination of network and task measures.

|                         |                                                                                | Model 1               | Model 2               | Model 3               |
|-------------------------|--------------------------------------------------------------------------------|-----------------------|-----------------------|-----------------------|
| Measure groups          | Task controls                                                                  | Measures only         | Fixed effects only    | Meas. & Fixed eff.    |
|                         | Network measures                                                               | All                   | All                   | All                   |
| <b>Controls</b>         | Intercept                                                                      | 2.37* (0.00121)       | 0.606* (0.000355)     | 1.51* (0.00135)       |
|                         | log <sub>10</sub> (Time step + 1)                                              | 0.166* (5.26e-05)     | 0.166* (5.3e-05)      | 0.166* (5.24e-05)     |
|                         | Team size                                                                      | 0.000915* (4.03e-05)  | -0.00145* (3.94e-05)  | -0.000871* (3.9e-05)  |
|                         | Team size <sup>2</sup>                                                         | -4.59e-05* (8.95e-07) | 2.09e-05* (8.74e-07)  | 5.44e-06* (8.63e-07)  |
|                         | log <sub>10</sub> (Search radius)                                              | 0.43* (0.000622)      | 0.211* (0.000489)     | 0.43* (0.000602)      |
| <b>Network measures</b> | Degree Cent. (Mean)                                                            | 0.145* (0.000367)     | -0.0283* (0.000327)   | 0.0429* (0.000362)    |
|                         | Degree Cent. (St. Dev.)                                                        | -0.00296* (0.000266)  | -0.00711* (0.000251)  | -0.00494* (0.00025)   |
|                         | Eigenvector Cent. (Mean)                                                       | 0.0399* (0.000484)    | 0.0183* (0.000471)    | 0.0215* (0.000465)    |
|                         | Eigenvector Cent. (St. Dev.)                                                   | -0.0173* (0.000541)   | 0.00778* (0.000523)   | -0.00463* (0.000521)  |
|                         | Betweenness Cent. (Mean)                                                       | -0.067* (0.000292)    | -0.014* (0.000274)    | -0.0342* (0.000278)   |
|                         | Betweenness Cent. (St. Dev.)                                                   | 0.0541* (0.000315)    | 0.00633* (0.000293)   | 0.0257* (0.000305)    |
|                         | Nearest Neighbor Degree (Mean)                                                 | -0.12* (0.000312)     | 0.00813* (0.000272)   | -0.044* (0.000292)    |
|                         | Nearest Neighbor Degree (St. Dev.)                                             | 0.00206* (0.000339)   | -0.00443* (0.000326)  | -0.00172* (0.000324)  |
|                         | Clustering Coeff.                                                              | 0.0491* (0.000183)    | -0.00109* (0.000135)  | 0.0195* (0.000174)    |
|                         | Degree Assortativity                                                           | 0.0338* (0.000441)    | -0.00577* (0.000426)  | 0.0103* (0.000427)    |
|                         | Shortest Path Length (Mean)                                                    | 0.103* (0.000847)     | 0.0259* (0.000799)    | 0.055* (0.000812)     |
|                         | Diameter                                                                       | -0.0728* (0.000933)   | -0.00214 (0.000888)   | -0.0303* (0.000893)   |
| <b>Task measures</b>    | Exploration difficulty (1 - Task integral)                                     | -0.571* (0.000161)    |                       | -0.533* (0.000535)    |
|                         | log <sub>10</sub> (Task number of peaks)                                       | 0.00379* (3.99e-06)   |                       | 0.00119* (5.07e-06)   |
|                         | Neighborhood alignment                                                         | -1.68* (0.00131)      |                       | -0.676* (0.00146)     |
|                         | Neighborhood interdependence                                                   | 0.16* (0.00028)       |                       | 0.0637* (0.000258)    |
| <b>Interactions</b>     | log <sub>10</sub> (Search radius) × Degree Cent. (Mean)                        | 0.0369* (0.000204)    | 0.0106* (0.000199)    | 0.0369* (0.000201)    |
|                         | log <sub>10</sub> (Search radius) × Degree Cent. (St. Dev.)                    | -0.00183* (0.000147)  | -0.00274* (0.000147)  | -0.00181* (0.000145)  |
|                         | log <sub>10</sub> (Search radius) × Eigenvector Cent. (Mean)                   | 0.0102* (0.000114)    | 0.0112* (0.000115)    | 0.0103* (0.000112)    |
|                         | log <sub>10</sub> (Search radius) × Eigenvector Cent. (St. Dev.)               | -0.0063* (0.000283)   | -0.00111* (0.000286)  | -0.00647* (0.000283)  |
|                         | log <sub>10</sub> (Search radius) × Betweenness Cent. (Mean)                   | -0.0196* (0.000161)   | -0.0126* (0.00016)    | -0.0197* (0.00016)    |
|                         | log <sub>10</sub> (Search radius) × Betweenness Cent. (St. Dev.)               | 0.017* (0.000176)     | 0.01* (0.000175)      | 0.0172* (0.000176)    |
|                         | log <sub>10</sub> (Search radius) × Nearest Neighbor Degree (Mean)             | -0.0342* (0.00017)    | -0.0151* (0.000165)   | -0.0342* (0.000166)   |
|                         | log <sub>10</sub> (Search radius) × Nearest Neighbor Degree (St. Dev.)         | 0.0012* (0.000198)    | 0.00021 (0.0002)      | 0.00119* (0.000197)   |
|                         | log <sub>10</sub> (Search radius) × Clustering Coeff.                          | 0.0132* (9.94e-05)    | 0.00563* (8.92e-05)   | 0.0132* (9.78e-05)    |
|                         | log <sub>10</sub> (Search radius) × Degree Assortativity                       | 0.0089* (0.000254)    | 0.00328* (0.000257)   | 0.0091* (0.000254)    |
|                         | log <sub>10</sub> (Search radius) × Shortest Path Length (Mean)                | 0.0322* (0.000466)    | 0.0222* (0.000465)    | 0.0323* (0.000464)    |
|                         | log <sub>10</sub> (Search radius) × Diameter                                   | -0.0214* (0.000512)   | -0.0113* (0.000513)   | -0.0214* (0.00051)    |
|                         | log <sub>10</sub> (Search radius) × Exploration difficulty (1 - Task integral) | 0.171* (8.26e-05)     | 0.198* (7.81e-05)     | 0.171* (8.15e-05)     |
|                         | log <sub>10</sub> (Search radius) × log <sub>10</sub> (Task number of peaks)   | -0.000562* (2.09e-06) | -0.000923* (1.65e-06) | -0.000563* (1.94e-06) |
|                         | log <sub>10</sub> (Search radius) × Neighborhood alignment                     | -0.459* (0.000699)    | -0.213* (0.000551)    | -0.459* (0.000676)    |
|                         | log <sub>10</sub> (Search radius) × Neighborhood interdependence               | 0.0433* (0.000152)    | 0.0203* (0.000107)    | 0.0432* (0.000147)    |
| <b>Statistics</b>       | Num. Observations                                                              | 55342898.0            | 55342898.0            | 55342898.0            |
|                         | R-squared (adj.)                                                               | 0.783937              | 0.79167               | 0.797693              |
|                         | AIC                                                                            | -8.67871e+07          | -8.8804e+07           | -9.04275e+07          |
|                         | BIC                                                                            | -8.67865e+07          | -8.8803e+07           | -9.04264e+07          |
|                         | F-statistic                                                                    | 6.24321e+06           | 3.73595e+06           | 3.86065e+06           |
|                         | F p-value                                                                      | < 0.001               | < 0.001               | < 0.001               |

**Table S2. Regression coefficients for models 1-3. Parenthetical statements show HC2 standard errors. Coefficients marked with an asterisk (\*) have  $p < 0.001$ , and all others have  $p > 0.01$ .**

|                         |                                                                                | Model 4               | Model 5               | Model 6               |
|-------------------------|--------------------------------------------------------------------------------|-----------------------|-----------------------|-----------------------|
| Measure groups          | Task controls                                                                  | Measures only         | Fixed effects only    | Meas. & Fixed eff.    |
|                         | Network measures                                                               | Disconn. only         | Disconn. only         | Disconn. only         |
| <b>Controls</b>         | Intercept                                                                      | 0.98* (0.000326)      | 0.609* (0.00031)      | 0.935* (0.000396)     |
|                         | log <sub>10</sub> (Time step + 1)                                              | 0.166* (4.93e-05)     | 0.166* (4.99e-05)     | 0.166* (4.9e-05)      |
|                         | Team size                                                                      | -0.000268* (3.69e-05) | -0.000858* (3.58e-05) | -0.000699* (3.53e-05) |
|                         | Team size <sup>2</sup>                                                         | -1.74e-05* (8.22e-07) | 9.24e-06* (7.99e-07)  | 2.84e-06* (7.84e-07)  |
|                         | log <sub>10</sub> (Search radius)                                              | 0.0456* (7.05e-05)    | 0.0253* (6.01e-05)    | 0.0456* (7.03e-05)    |
| <b>Network measures</b> | Degree Cent. (Mean)                                                            | -0.0468* (0.000266)   | -0.0263* (0.000254)   | -0.0342* (0.000246)   |
|                         | Degree Cent. (St. Dev.)                                                        | 0.0161* (0.000245)    | -0.011* (0.000222)    | 0.00208* (0.000226)   |
|                         | Eigenvector Cent. (Mean)                                                       | 0.0109* (0.000428)    | 0.0128* (0.000416)    | 0.00923* (0.000409)   |
|                         | Eigenvector Cent. (St. Dev.)                                                   | 0.00985* (0.000337)   | 0.00719* (0.000279)   | 0.00733* (0.000319)   |
|                         | Betweenness Cent. (Mean)                                                       | 0.0215* (0.000212)    | -0.00243* (0.000142)  | 0.00884* (0.000197)   |
|                         | Betweenness Cent. (St. Dev.)                                                   | -0.0207* (0.000247)   | 0.00693* (0.000211)   | -0.00614* (0.000231)  |
|                         | Nearest Neighbor Degree (Mean)                                                 | 0.0233* (0.000241)    | 0.0064* (0.000211)    | 0.0137* (0.000224)    |
|                         | Nearest Neighbor Degree (St. Dev.)                                             | -0.0139* (0.000282)   | 0.00163* (0.000267)   | -0.00542* (0.000263)  |
|                         | Clustering Coeff.                                                              | -0.0118* (0.000152)   | -0.000998* (0.000114) | -0.00579* (0.000141)  |
|                         | Degree Assortativity                                                           |                       |                       |                       |
|                         | Shortest Path Length (Mean)                                                    |                       |                       |                       |
|                         | Diameter                                                                       |                       |                       |                       |
| <b>Task measures</b>    | Exploration difficulty (1 - Task integral)                                     | -0.531* (0.000143)    |                       | -0.511* (0.000396)    |
|                         | log <sub>10</sub> (Task number of peaks)                                       | 0.00314* (3.92e-06)   |                       | 0.000977* (4.69e-06)  |
|                         | Neighborhood alignment                                                         | -0.0936* (0.000204)   |                       | -0.0429* (0.000192)   |
|                         | Neighborhood interdependence                                                   | 0.0932* (0.00021)     |                       | 0.0426* (0.000202)    |
| <b>Interactions</b>     | log <sub>10</sub> (Search radius) × Degree Cent. (Mean)                        | -0.0158* (0.000147)   | -0.013* (0.000149)    | -0.0158* (0.000145)   |
|                         | log <sub>10</sub> (Search radius) × Degree Cent. (St. Dev.)                    | 0.00255* (0.000136)   | -0.0029* (0.000133)   | 0.00257* (0.000134)   |
|                         | log <sub>10</sub> (Search radius) × Eigenvector Cent. (Mean)                   | 0.00416* (8.2e-05)    | 0.00663* (7.89e-05)   | 0.00418* (8.1e-05)    |
|                         | log <sub>10</sub> (Search radius) × Eigenvector Cent. (St. Dev.)               | 0.00279* (0.000162)   | 0.00208* (0.000148)   | 0.00261* (0.000161)   |
|                         | log <sub>10</sub> (Search radius) × Betweenness Cent. (Mean)                   | 0.00569* (0.000117)   | 0.000159 (0.000101)   | 0.00559* (0.000116)   |
|                         | log <sub>10</sub> (Search radius) × Betweenness Cent. (St. Dev.)               | -0.00419* (0.000138)  | 0.00191* (0.000133)   | -0.00405* (0.000137)  |
|                         | log <sub>10</sub> (Search radius) × Nearest Neighbor Degree (Mean)             | 0.00492* (0.000134)   | 0.00153* (0.00013)    | 0.00482* (0.000132)   |
|                         | log <sub>10</sub> (Search radius) × Nearest Neighbor Degree (St. Dev.)         | -0.00224* (0.000163)  | 0.000544* (0.000164)  | -0.00225* (0.000162)  |
|                         | log <sub>10</sub> (Search radius) × Clustering Coeff.                          | -0.00357* (8.54e-05)  | -0.00206* (7.67e-05)  | -0.00361* (8.43e-05)  |
|                         | log <sub>10</sub> (Search radius) × Degree Assortativity                       |                       |                       |                       |
|                         | log <sub>10</sub> (Search radius) × Shortest Path Length (Mean)                |                       |                       |                       |
|                         | log <sub>10</sub> (Search radius) × Diameter                                   |                       |                       |                       |
|                         | log <sub>10</sub> (Search radius) × Exploration difficulty (1 - Task integral) | 0.183* (7.45e-05)     | 0.216* (7.27e-05)     | 0.183* (7.49e-05)     |
|                         | log <sub>10</sub> (Search radius) × log <sub>10</sub> (Task number of peaks)   | -0.000739* (2.02e-06) | -0.00101* (1.58e-06)  | -0.000739* (1.85e-06) |
|                         | log <sub>10</sub> (Search radius) × Neighborhood alignment                     | -0.0262* (0.000112)   | -0.00788* (7.71e-05)  | -0.0261* (0.000111)   |
|                         | log <sub>10</sub> (Search radius) × Neighborhood interdependence               | 0.026* (0.000118)     | 0.00877* (8.28e-05)   | 0.0259* (0.000117)    |
| <b>Statistics</b>       | Num. Observations                                                              | 63648000.0            | 63648000.0            | 63648000.0            |
|                         | R-squared (adj.)                                                               | 0.77444               | 0.785493              | 0.792898              |
|                         | AIC                                                                            | -9.75632e+07          | -1.00761e+08          | -1.02997e+08          |
|                         | BIC                                                                            | -9.75627e+07          | -1.0076e+08           | -1.02996e+08          |
|                         | F-statistic                                                                    | 8.46353e+06           | 4.39242e+06           | 4.66763e+06           |
|                         | F p-value                                                                      | < 0.001               | < 0.001               | < 0.001               |

**Table S3. Regression coefficients for models 4-6. Parenthetical statements show HC2 standard errors. Coefficients marked with an asterisk (\*) have  $p < 0.001$ , and all others have  $p > 0.01$ .**

| Network type                       | Degree Cent. (Mean) | Degree Cent. (St. Dev.) | Eigenvector Cent. (Mean) | Eigenvector Cent. (St. Dev.) | Betweenness Cent. (Mean) | Betweenness Cent. (St. Dev.) | Nearest Neighbor Degree (Mean) | Nearest Neighbor Degree (St. Dev.) | Clustering Coeff. | Degree Assortativity | Shortest Path Length (Mean) | Diameter |
|------------------------------------|---------------------|-------------------------|--------------------------|------------------------------|--------------------------|------------------------------|--------------------------------|------------------------------------|-------------------|----------------------|-----------------------------|----------|
| Complete                           | 1.000               | 0.000                   | 0.200                    | 0.000                        | 0.000                    | 0.000                        | 1.000                          | 0.000                              | 1.000             | 0.000                | 1.000                       | 1.000    |
| Empty (Indiv. Learning)            | 0.000               | 0.000                   | 0.200                    | 0.000                        | 0.000                    | 0.000                        | 0.000                          | 0.000                              | 0.000             |                      |                             |          |
| Pref. Attach. ( $m = 2, p = 0.1$ ) | 0.153               | 0.106                   | 0.175                    | 0.099                        | 0.056                    | 0.095                        | 0.253                          | 0.081                              | 0.321             | -0.305               | 2.289                       | 4.124    |
| Pref. Attach. ( $m = 2, p = 0.5$ ) | 0.153               | 0.111                   | 0.174                    | 0.101                        | 0.058                    | 0.110                        | 0.261                          | 0.081                              | 0.512             | -0.302               | 2.327                       | 4.284    |
| Pref. Attach. ( $m = 2, p = 0.9$ ) | 0.153               | 0.116                   | 0.173                    | 0.103                        | 0.060                    | 0.131                        | 0.271                          | 0.085                              | 0.686             | -0.315               | 2.387                       | 4.428    |
| Random ( $p = 0.1$ )               | 0.101               | 0.059                   | 0.158                    | 0.123                        | 0.075                    | 0.087                        | 0.128                          | 0.050                              | 0.072             | -0.110               | 3.085                       | 6.917    |
| Random ( $p = 0.5$ )               | 0.500               | 0.100                   | 0.196                    | 0.038                        | 0.022                    | 0.011                        | 0.521                          | 0.022                              | 0.501             | -0.085               | 1.501                       | 2.164    |
| Random ( $p = 0.9$ )               | 0.901               | 0.059                   | 0.200                    | 0.012                        | 0.004                    | 0.001                        | 0.905                          | 0.006                              | 0.901             | -0.080               | 1.099                       | 2.000    |
| Ring                               | 0.083               | 0.000                   | 0.200                    | 0.000                        | 0.239                    | 0.000                        | 0.083                          | 0.000                              | 0.000             | 0.000                | 6.500                       | 12.000   |
| Ring of Cliques                    | 0.183               | 0.021                   | 0.199                    | 0.020                        | 0.094                    | 0.118                        | 0.186                          | 0.002                              | 0.840             | -0.100               | 3.167                       | 5.000    |
| Rook's Graph                       | 0.333               | 0.000                   | 0.200                    | 0.000                        | 0.029                    | 0.000                        | 0.333                          | 0.000                              | 0.429             | 0.000                | 1.667                       | 2.000    |
| Small World ( $k = 2, p = 0.1$ )   | 0.083               | 0.017                   | 0.162                    | 0.111                        | 0.214                    | 0.131                        | 0.088                          | 0.012                              | 0.010             | -0.074               | 6.512                       | 16.238   |
| Small World ( $k = 2, p = 0.5$ )   | 0.083               | 0.036                   | 0.155                    | 0.127                        | 0.149                    | 0.158                        | 0.103                          | 0.027                              | 0.024             | -0.220               | 5.176                       | 12.441   |
| Small World ( $k = 2, p = 0.9$ )   | 0.083               | 0.042                   | 0.152                    | 0.131                        | 0.137                    | 0.161                        | 0.109                          | 0.033                              | 0.025             | -0.230               | 4.715                       | 10.952   |
| Star                               | 0.080               | 0.192                   | 0.167                    | 0.112                        | 0.040                    | 0.200                        | 0.962                          | 0.192                              | 0.000             | -1.000               | 1.920                       | 2.000    |
| Tree                               | 0.080               | 0.039                   | 0.158                    | 0.124                        | 0.183                    | 0.207                        | 0.104                          | 0.030                              | 0.000             | -0.250               | 5.198                       | 12.208   |
| Wheel                              | 0.160               | 0.175                   | 0.177                    | 0.095                        | 0.037                    | 0.174                        | 0.405                          | 0.058                              | 0.643             | -0.333               | 1.840                       | 2.000    |
| Windmill                           | 0.200               | 0.167                   | 0.181                    | 0.086                        | 0.035                    | 0.174                        | 0.367                          | 0.042                              | 0.965             | -0.250               | 1.800                       | 2.000    |

**Table S4.** Mean values of each network measure for each type of network for teams of  $n = 9$ .

334 **SI Dataset S1 (execset010\_model3xx\_team\_is\_nbhd.pickle.gz)**

| Variable                                  | Description                                                                                                                                                          |
|-------------------------------------------|----------------------------------------------------------------------------------------------------------------------------------------------------------------------|
| team_size                                 | Number of agents in the team                                                                                                                                         |
| team_graph_type                           | The type of network                                                                                                                                                  |
| team_fn_type                              | The type of task                                                                                                                                                     |
| agent_steplim                             | The allowed search radius                                                                                                                                            |
| run_step                                  | The run number indicating the time step in that execution of the model                                                                                               |
| team_graph_centrality_degree_mean         | The mean of the degree centralities of the agents                                                                                                                    |
| team_graph_centrality_degree_stddev       | The standard deviation of the degree centralities of the agents                                                                                                      |
| team_graph_centrality_eigenvector_mean    | The mean of the eigenvector centralities of the agents                                                                                                               |
| team_graph_centrality_eigenvector_stddev  | The standard deviation of the eigenvector centralities of the agents                                                                                                 |
| team_graph_centrality_betweenness_mean    | The mean of the betweenness centralities of the agents                                                                                                               |
| team_graph_centrality_betweenness_stddev  | The standard deviation of the betweenness centralities of the agents                                                                                                 |
| team_graph_nearest_neighbor_degree_mean   | The mean of the nearest neighbor degrees of each agent                                                                                                               |
| team_graph_nearest_neighbor_degree_stddev | The standard deviation of the nearest neighbor degrees of each agent                                                                                                 |
| team_graph_clustering                     | The clustering coefficient of the team network                                                                                                                       |
| team_graph_assortativity                  | The degree assortativity of the team network                                                                                                                         |
| team_graph_pathlength                     | The mean shortest path length of the team network                                                                                                                    |
| team_graph_diameter                       | The largest shortest path length of the team network                                                                                                                 |
| team_fn_diff_integral                     | The exploration difficulty of the task                                                                                                                               |
| team_fn_diff_peaks                        | The exploitation difficulty of the task                                                                                                                              |
| team_fn_alignment                         | The alignment between task neighborhoods                                                                                                                             |
| team_fn_interdep                          | The interdependence between task neighborhoods                                                                                                                       |
| team_performance                          | The team's performance at the specific time                                                                                                                          |
| team_productivity                         | The team productivity at that run step, measured as the difference between the performance at the current time and the prior time, then divided by the the team size |
| team_fn_weight                            | The weighting type used in the task, if applicable                                                                                                                   |
| team_fn_frequency                         | The frequency type used in the task, if applicable                                                                                                                   |
| team_fn_exponent                          | The exponent type used in the task, if applicable                                                                                                                    |
| team_fn                                   | A string combining the other team_fn_fields                                                                                                                          |

336 **SI Dataset S2 (execset010\_stats.pickle.gz)**

337 **SI Dataset S3 (execset010\_stats\_by\_graph.pickle.gz)**

| Variable   | Description                                                                                                             |
|------------|-------------------------------------------------------------------------------------------------------------------------|
| ci_lo      | Lower bound of the 95% confidence interval for the specified statistic                                                  |
| ci_hi      | Upper bound of the 95% confidence interval for the specified statistic                                                  |
| diff_mean  | Absolute difference between the mean of the empty graph and the network type shown with all other parameters held fixed |
| diff_ci_lo | Lower bound of the 95% confidence interval for the absolute difference between means                                    |
| diff_ci_hi | Upper bound of the 95% confidence interval for the absolute difference between means                                    |
| pct_mean   | Percent difference between the mean of the empty graph and the network type shown with all other parameters held fixed  |
| pct_ci_lo  | Lower bound of the 95% confidence interval for the percent difference between means                                     |
| pct_ci_hi  | Upper bound of the 95% confidence interval for the percent difference between means                                     |

339 **SI Dataset S4 (execset010\_by\_graph\_vs\_empty.pickle.gz)**

340 **SI Dataset S5 (execset010\_vs\_empty.pickle.gz)**

341 **References**

- 342 1. JE McGrath, *Groups: Interaction and Performance*. (Prentice-Hall Englewood Cliffs, NJ) Vol. 14, (1984).
- 343 2. AW Woolley, CF Chabris, A Pentland, N Hashmi, TW Malone, Evidence for a collective intelligence factor in the  
344 performance of human groups. *Science* **330**, 686–688 (2010).
- 345 3. C Riedl, YJ Kim, P Gupta, TW Malone, AW Woolley, Quantifying collective intelligence in human groups. *Proc. Natl.*  
346 *Acad. Sci.* **118** (2021).
- 347 4. K Lewis, B Herndon, Transactive memory systems: Current issues and future research directions. *Organ. Sci.* **22**,  
348 1254–1265 (2011).
- 349 5. DG Bachrach, et al., Transactive memory systems in context: A meta-analytic examination of contextual factors in  
350 transactive memory systems development and team performance. *J. Appl. Psychol.* **104**, 464–493 (2019).
- 351 6. JW Rivkin, N Siggelkow, Patterned interactions in complex systems: Implications for exploration. *Manag. Sci.* **53**,  
352 1068–1085 (2007).

- 353 7. D Barkoczi, M Galesic, Social learning strategies modify the effect of network structure on group performance. *Nat.*  
354 *Commun.* **7**, 13109–13109 (2016).
- 355 8. A Almaatouq, M Alsobay, M Yin, DJ Watts, Task complexity moderates group synergy. *Proc. Natl. Acad. Sci.* **118** (2021).
- 356 9. P Virtanen, et al., SciPy 1.0: Fundamental algorithms for scientific computing in python. *Nat. Methods* **17**, 261–272  
357 (2020).
- 358 10. S Surjanovic, D Bingham, Virtual library of simulation experiments: Test functions and datasets (2013).
- 359 11. M Newman, *Networks*. (Oxford university press), (2018).
- 360 12. AA Hagberg, DA Schult, PJ Swart, Exploring network structure, dynamics, and function using NetworkX in *Proceedings*  
361 *of the 7th Python in Science Conference*, eds. G Varoquaux, T Vaught, J Millman. (Pasadena, CA USA), pp. 11–15 (2008).
- 362 13. J Shore, E Bernstein, D Lazer, Facts and figuring: An experimental investigation of network structure and performance in  
363 information and solution spaces. *Organ. Sci.* **26**, 1432–1446 (2015).
- 364 14. WS Lovejoy, A Sinha, Efficient structures for innovative social networks. *Manag. Sci.* **56**, 1127–1145 (2010).
- 365 15. C Fang, J Lee, MA Schilling, Balancing exploration and exploitation through structural design: The isolation of subgroups  
366 and organizational learning. *Organ. Sci.* **21**, 625–642 (2010).
- 367 16. SD Dionne, H Sayama, FJ Yammarino, Diversity and social network structure in collective decision making: Evolutionary  
368 perspectives with agent-based simulations. *Complexity* **2019**, e7591072 (2019).
- 369 17. J Meluso, J Austin-Breneman, JP Bagrow, L Hébert-Dufresne, A review and framework for modeling complex engineered  
370 system development processes. *IEEE Transactions on Syst. Man, Cybern. Syst.* pp. 1–13 (2022).
- 371 18. P Holme, BJ Kim, Growing scale-free networks with tunable clustering. *Phys. review E* **65**, 26107–26107 (2002).
- 372 19. R Laskar, C Wallis, Chessboard graphs, related designs, and domination parameters. *J. Stat. Plan. Inference* **76**, 285–294  
373 (1999).
- 374 20. F Pedregosa, et al., Scikit-learn: Machine learning in python. *J. Mach. Learn. Res.* **12**, 2825–2830 (2011).
- 375 21. S Oldham, et al., Consistency and differences between centrality measures across distinct classes of networks. *PLOS ONE*  
376 **14**, e0220061 (2019).
- 377 22. S Seabold, J Perktold, Statsmodels: Econometric and statistical modeling with python in *Proceedings of the 9th Python in*  
378 *Science Conference*. (Austin, TX), Vol. 57, pp. 10–25080 (2010).
